# Supplementary material for: Online Resource Allocation with Stochastic Resource Consumption
Source: arXiv:2012.07933 source file (2020-12-18)
Supplement: Supplementary file 1 [file Online_Resource_Allocatoin_with_Stochastic_Consumption.pdf]

# Online Resource Allocation with Stochastic Resource Consumption

Jiashuo Jiang    Jiawei Zhang

Department of Technology, Operations & Statistics, Stern School of Business, New York University

**Abstract:** we consider an online resource allocation problem where multiple resources, each with an individual initial capacity, are available to serve random requests arriving sequentially over multiple discrete time periods. At each time period, one request arrives and its associated reward and size are drawn independently from a known distribution stationary across time. Upon its arrival and revealing itself, an online decision has to be made on whether or not to accept the request. If accepted, another online decision should also be made to specify on assigning which resource to serve the request, then a certain amount of the resource equal to the size will be consumed and a reward will be collected. The objective of the decision maker is to maximize the total collected reward subject to the capacity constraints. For a general model where both the size and the reward of each request depend on the resource assigned, we propose a non-adaptive threshold policy with a competitive ratio 0.302 and show that no online algorithm could achieve a ratio better than 0.5. We then propose an adaptive threshold policy and show that when the reward distribution has a finite support, our policy enjoys an optimal  $O(\log T)$  regret bound, where  $T$  denotes the total time periods. When the support of the reward distribution is not finite, we develop another adaptive threshold policy with a  $O(\log T)$  regret bound when both the reward and the size of each request are resource-independent.

---

## 1. Introduction

We study a general online resource allocation problem where multiple resources, each with an initial individual capacity, are available to serve a stream of requests arriving over a horizon of finite time periods. At each period, one request arrives with an associated reward and size, whose values are assumed to be random, following a given probability distribution that could be resource-dependent. Upon the arrival of a request, its reward and size are revealed. Then a decision-maker has to irrevocably decide to reject or accept it and to assign an available resource to serve it if accepted. If a request is served by a resource, a reward is collected and a certain amount of the resource equal to the size is consumed. The decision maker's objective is to maximize the total collected reward without violating the resource capacity constraints.

Our model generalizes several problems studied in the previous literature. For example, the single-resource case of our model reduces to the online knapsack problem, which has a wide range of applications in logistics and pricing among others, as described in Papastavrou et al. (1996). For the multi-resource case, by assuming that the reward is equal to the size for every request, our model reduces to the service reservation problem studied in Stein et al. (2019), which is also called

the online adwords problem (e.g. Goel and Mehta (2008)) if each request is allowed to be served partially. If the sizes of the requests are all equal to 1, then our model becomes the online matching problem (e.g. Feldman et al. (2009)). Note that the online knapsack problem, online adwords problem and online matching problem have also been applied extensively in online advertising (e.g. Zhou et al. (2008), Mehta et al. (2005), Mehta (2013)). In all these problems, the requests could arrive in an adversary order (e.g. Zhou et al. (2008), Ma et al. (2019), Karp et al. (1990)) or in a stochastic order (e.g. Papastavrou et al. (1996), Stein et al. (2019), Feldman et al. (2009)). Our model assumes a stationary stochastic arriving order, i.e., the values of the reward and size of every request are drawn independently from a known distribution which is stationary across time.

The objective of our paper is to develop near optimal policies for our model. Throughout the paper, we will compare the performance of our policies to the prophet, i.e., the optimal offline decision maker. We will measure the performance of our policies in different ways. One is to bound the so-called *competitive ratio*, which is concerned about the *relative* expected difference between our policy and the prophet, while the other one is to bound the *regret*, which is concerned about the *additive* expected difference. The formal definitions of competitive ratio and regret will be provided in Section 2 after introducing the problem formulation and notations.

### 1.1. Main Results and Contributions

We first analyze the general model where both the size and the reward of each request are resource-dependent. We propose a non-adaptive threshold policy and we show that our policy enjoys a competitive ratio of 0.302, which is the first constant competitive ratio for this general model. In contrast, previous papers only focused on some specific settings to obtain constant competitive ratios. For example, for the service reservation problem in Stein et al. (2019), they obtained a 0.321 competitive ratio when the requests arrive according to a known Poisson process. For the online matching problem, Feldman et al. (2009) obtained a 0.67 competitive ratio under stationary stochastic input and Brubach et al. (2016) improved to 0.705. For the single-resource case, Dütting et al. (2017) obtained a 0.2 competitive ratio under non-stationary stochastic input. Moreover, we show that 0.5 is the upper bound of the competitive ratio for any online policy, thus the competitive ratio of our policy is close to the optimum.

Our non-adaptive policy is based on constructing a linear programming to serve as an upper bound of the expected reward obtained by the prophet, and we will use its optimal solution to randomly route each request to a resource. Then, for each resource, instead of accepting all the routed requests, we will classify the routed requests into two categories based on the size and we will allow the resource to only serve one particular category of the routed requests. By doing so, we will have a control over the size of the accepted requests and then based on this feature, we could derive a

lower bound of the expected reward obtained by our policy. Note that a similar procedure is also adopted by Stein et al. (2019) to develop their policy. The main difference is that in their model, the reward is assumed to be equal to the size, thus they only need to lower bound the expected capacity utilization of their policy. However, in our model, the reward could be arbitrarily different from the size, which would require different technics to lower bound the expected reward of the proposed policy.

Then, we focus on the setting where the total number of the requests is large. We will consider this setting by assuming either the reward distribution has a finite support or both the reward and the size of each request are resource-independent. Under each assumption, we propose an adaptive threshold policy which enjoys a  $O(\log T)$  regret bound, where  $T$  denotes the total time periods. Our results generalize the  $O(\log T)$  regret bound in Arlotto and Xie (2020) from the single-resource case where the reward is unitary to the multi-resource case where the reward could take multiple values. Also the numerical experiments and discussions in Arlotto and Xie (2020) showed that the  $O(\log T)$  regret bound is of optimal order even for the single-resource unitary-reward case, thus our regret bound is order tight. Note that while all these results assume that the size distribution is continuous, some other papers assumed that both the reward distribution and the size distribution have a finite support and obtained uniform regret bound (e.g. Bumpensanti and Wang (2020), Arlotto and Gurvich (2019), Vera and Banerjee (2019), Vera et al. (2019), Freund and Banerjee (2019)). However, their uniform regret bound will depend implicitly on the cardinality of the support of the reward and size, thus their methods and results could not be generalized to our setting where the size distribution is assumed to be a continuous distribution.

Our approach is based on showing that under our assumptions, the optimal solution of the linear programming prophet upper bound possesses a threshold structure, thus we could mimic the prophet by following an adaptive threshold policy. Also, we show that the corresponding thresholds could be given in a closed-form expression and we further show that this expression would enable us to characterize the convex structural property of the thresholds, which will finally lead to the regret bound of our policy. Note that for the single-resource unitary-reward case, our prophet upper bound is identical to the upper bound in Arlotto and Xie (2020). However, as discussed in Section 3, their approach to derive the prophet upper bound is based on an observation that doesn't hold under more general setting thus prohibits them from extending their results. Instead, our approach directly deals with the linear programming upper bound of the prophet and thus gets over this prohibition. As a result, we could affirmatively answer the open problem left in Section 8 of Arlotto and Xie (2020) that whether the  $O(\log T)$  regret bound holds when the reward could take multiple values, and we even generalize to the multi-resource case. Moreover, by studying how the expected reward obtained by the prophet scales over  $T$ , we establish the asymptotic optimality of our policies when  $T \rightarrow \infty$ .

## 1.2. Other Related Literature

Our model generalizes the online knapsack problem and the online matching problem, and is also closely related to the online adwords problem. We will briefly review the literature on these problems as follows.

For the online knapsack problem, when the requests arrive in an adversary order, Marchetti-Spaccamela and Vercellis (1995) showed that there doesn't exist an online algorithm with constant competitive ratio. Thus, Marchetti-Spaccamela and Vercellis (1995) and a following work Lueker (1998) devoted to studying the regret bound of the online knapsack problem. Later on, by assuming the size of each request is very small compared to the knapsack capacity and the reward/size ratio of each request is lower bounded and upper bounded by two positive constant  $L$  and  $U$ , Zhou et al. (2008) obtained a competitive ratio of  $\log(U/L) + 1$  under adversary input and further generalized their method to the multiple-choice knapsack problem to obtain a competitive ratio of  $\log(U/L) + 2$ . Finally, Alaei et al. (2013) studied an online stochastic generalized assignment problem, which is a multi-dimensional generalization of the online knapsack problem. They obtained a competitive ratio of  $1 - \frac{1}{\sqrt{k}}$  under stochastic input when the size of the request is upper bounded by  $1/k$  fraction of the capacity of each resource. However, no online algorithm could achieve a constant competitive ratio when  $k = 1$ .

The literature of the online matching problem is extensive and we will refer interested readers to the survey by Mehta (2013). There is also considerable recent works devoting to various generalizations of the online matching problem, which involves the setting where one could offer an assortment of resources to each arrival (e.g. Golrezaei et al. (2014), Ma et al. (2018), Ma and Simchi-Levi (2019)) and the setting where the allocated resource is only used for a duration and then could be re-allocated (e.g. Rusmevichientong et al. (2020), Goyal et al. (2020)).

For the online adwords problem, a common assumption in the literature is that the size of each request is very small compared to the capacity of each resource and various results were obtained under this assumption. For example, it is shown in Mehta et al. (2005) that a greedy algorithm which assigns each request to the resource with highest reward has a competitive ratio of 0.5 under adversarial input and then it is shown in Goel and Mehta (2008) that this greedy algorithm enjoys a tight competitive ratio  $1 - 1/e$  under the random permutation input. Also, Mehta et al. (2005) proposed a deterministic algorithm which enjoys an optimal competitive ratio of  $1 - 1/e$  under adversarial input and later on, Mirrokni et al. (2012) showed that this algorithm has a competitive ratio of 0.76 under random permutation input. Asymptotic competitive ratios are also considered in the literature. For example, when the size of each request is smaller than  $1/k$  fraction of the capacity, Devanur et al. (2012) proved a competitive ratio of  $1 - \frac{1}{\sqrt{2\pi k}}$  when the requests were

drawn repeatedly from a common distribution which is not necessarily known in advance.

Our problem is also related to the Online Linear Programming (OLP) literature. The OLP problem takes a standard linear programming as the underlying form, while the columns of the constraint matrix and the corresponding coefficients of the objective function will arrive sequentially over time. Much effort has been devoted to studying the trade-off between algorithm competitiveness and resource capacity, denoted as  $c$ , (e.g. Devanur and Hayes (2009), Molinaro and Ravi (2013), Agrawal et al. (2014), Kesselheim et al. (2014)) and it is shown that in order to have a  $1 - \varepsilon$  competitive ratio, it is essential for  $c$  to be at least  $\Omega(1/\varepsilon^2)$ , which implies that it is necessary for  $c$  to be scaled up simultaneously with  $T$  to have any regret bound sublinear in the prophet. Also, a recent work Li and Ye (2019) adopted an asymptotic setting that  $c$  scales up linearly in  $T$  and proved a  $O(\log T \log \log T)$  regret bound. However, a term  $\frac{T}{c}$  shows up in their regret bound and is abbreviated in notation  $O(\cdot)$  since it is a constant in their framework. As a result, a direct application of their result to our problem would imply a regret at least linear in  $T$  since we will consider our problem under the setting that  $c$  is fixed as  $T \rightarrow \infty$ . The above discussions imply that, although the formulation of OLP seems like a non-parametric generalization of our model, the fixed resource capacity setting considered in this paper will finally differentiate our problem from OLP and would require analysis other than those in OLP literature. Thus, though closely related, our work is not covered by the OLP literature and serves as a supplement to online decision making literature under an asymptotic setting other than that of OLP literature.

## 2. Problem Formulation

In our problem, there are  $m$  resources. Each resource  $j$  has an initial capacity  $c_j$ . The resources are used to serve a stream of requests arriving sequentially over  $T$  discrete time periods. At each time period  $t$ , one request arrives, denoted as request  $t$ , which is associated with a nonnegative reward  $\tilde{\mathbf{r}}^t = [\tilde{r}_1^t, \tilde{r}_2^t, \dots, \tilde{r}_m^t]$  and a positive size  $\tilde{\mathbf{d}}^t = [\tilde{d}_1^t, \tilde{d}_2^t, \dots, \tilde{d}_m^t]$ . Here,  $(\tilde{\mathbf{r}}^t, \tilde{\mathbf{d}}^t)$  is assumed to be stochastic and its value is drawn independently from a known distribution  $F(\cdot)$ , which is stationary across time. After the value of  $(\tilde{\mathbf{r}}^t, \tilde{\mathbf{d}}^t)$  is revealed, denoted separately as  $\mathbf{r}^t = [r_1^t, r_2^t, \dots, r_m^t]$  and  $\mathbf{d}^t = [d_1^t, d_2^t, \dots, d_m^t]$ , the decision maker has to irrevocably decide to reject or accept request  $t$ . If rejected, no resource will be consumed and no reward will be collected. If accepted, the decision maker has to assign one of the resources to serve it. If resource  $j$  is assigned to serve request  $t$ , then  $d_j^t$  units of resource  $j$  will be consumed and a reward  $r_j^t$  will be collected. The objective of the decision maker is to maximize the total collected reward without violating the capacity constraints. Without loss of generality, we only focus on the case that both the reward and the size of each request are bounded. Moreover, note that if the size of a request exceeds the initial capacity of a resource, then this request could never be served by this resource and the corresponding reward could never be collected. Thus, throughout the paper, we will make the following assumption:

**Assumption 1** *There exists  $\bar{d}$  and  $\bar{r}$  such that for every realization  $(\mathbf{r}, \mathbf{d})$  and every  $j$ , the following two conditions hold: (1)  $\bar{d} \geq d_j > 0$  and  $\bar{r} \geq r_j \geq 0$ ; (2)  $d_j > c_j$  implies that  $r_j = 0$ .*

Any policy  $\pi$  is defined via a sequence of binary variables  $\{x_j^\pi(t)\}$ , where  $x_j^\pi(t)$  denotes whether request  $t$  is served by resource  $j$ . Here,  $x_j^\pi(t)$  is random and its realization is dependent on the arriving sequence of the requests. Policy  $\pi$  is feasible as long as  $\pi$  is non-anticipating, i.e., for any  $j$ ,  $x_j^\pi(t)$  can only depend on  $\{(\mathbf{r}^1, \mathbf{d}^1), (\mathbf{r}^2, \mathbf{d}^2), \dots, (\mathbf{r}^t, \mathbf{d}^t)\}$ , and  $\pi$  satisfies the following constraints:

$$\sum_{t=1}^T d_j^t \cdot x_j^\pi(t) \leq c_j \quad \forall j \quad \text{and} \quad \sum_{j=1}^m x_j^\pi(t) \leq 1 \quad \forall t \quad (1)$$

The total reward collected by policy  $\pi$  is denoted as:

$$V^\pi(\mathbf{I}) = \sum_{t=1}^T \sum_{j=1}^m r_j^t \cdot x_j^\pi(t) \quad (2)$$

where  $\mathbf{I} = \{(\mathbf{r}^1, \mathbf{d}^1), (\mathbf{r}^2, \mathbf{d}^2), \dots, (\mathbf{r}^T, \mathbf{d}^T)\}$  denotes the sample path of request arrivals over the entire time horizon. Then the expected total reward collected by the policy  $\pi$  is denoted as  $\mathbb{E}[V^\pi(\mathbf{I})]$ , where  $\mathbb{E}[\cdot]$  denotes taking expectation over the request arrivals  $\mathbf{I}$ .

We compare the performance of any feasible policy  $\pi$  to the prophet, an offline decision maker with full knowledge of the arriving sequence of the requests and always applying the optimal policy in hindsight. Similarly, given the sample path  $\mathbf{I}$ , we use a binary variable  $x_j^t(\mathbf{I})$  to denote whether request  $t$  is served by resource  $j$  under the optimal policy in hindsight. Here,  $x_j^t(\mathbf{I})$  is allowed to depend on the whole sample path  $\mathbf{I}$ . Indeed, given  $\mathbf{I}$ ,  $\{x_j^t(\mathbf{I})\}$  is the optimal solution to the following optimal offline problem:

$$\begin{aligned} V^{\text{off}}(\mathbf{I}) = \max \quad & \sum_{t=1}^T \sum_{j=1}^m r_j^t \cdot x_j^t \\ \text{s.t.} \quad & \sum_{t=1}^T d_j^t \cdot x_j^t \leq c_j \quad \forall j \\ & \sum_{j=1}^m x_j^t \leq 1 \quad \forall t \\ & x_j^t \in \{0, 1\} \quad \forall j, \forall t \end{aligned} \quad (3)$$

Then, the expected total reward collected by the prophet is denoted as  $\mathbb{E}[V^{\text{off}}(\mathbf{I})]$ .

We now introduce *competitive ratio* and *regret* to measure the performance of the policy  $\pi$ . A feasible policy  $\pi$  is called to have a competitive ratio  $\alpha$  if

$$\mathbb{E}[V^\pi(\mathbf{I})] \geq \alpha \cdot \mathbb{E}[V^{\text{off}}(\mathbf{I})] \quad (4)$$

holds for all model parameters. And the regret of the policy  $\pi$ , denoted as  $\text{Regret}(\pi)$ , is defined as the difference between the expected total reward collected by the prophet and the expected total reward collected by the policy  $\pi$ :

$$\text{Regret}(\pi) = \mathbb{E}[V^{\text{off}}(\mathbf{I})] - \mathbb{E}[V^\pi(\mathbf{I})] \quad (5)$$

### 3. Non-adaptive Threshold Policy and Competitive Ratio Bound

In this section, we propose a nonadaptive threshold policy for our problem and prove the corresponding 0.302 competitive ratio. Since the hindsight optimum obtained by solving the integer programming (3) often preserves complex structure and thus is very hard to analyze, we will first derive a tractable upper bound of  $\mathbb{E}[V^{\text{off}}(\mathbf{I})]$ . Then based on our prophet upper bound, we will derive our policy and prove the competitive ratio bound. The upper bound could be formulated as the following linear programming (LP):

$$\begin{aligned} \text{LP}^{\text{UB}} := \max \quad & T \cdot \mathbb{E}\left[\sum_{j=1}^m r_j \cdot x_j(\mathbf{r}, \mathbf{d})\right] \\ \text{s.t.} \quad & T \cdot \mathbb{E}[d_j \cdot x_j(\mathbf{r}, \mathbf{d})] \leq c_j \quad \forall j \\ & \sum_{j=1}^m x_j(\mathbf{r}, \mathbf{d}) \leq 1 \quad \forall (\mathbf{r}, \mathbf{d}) \\ & 0 \leq x_j(\mathbf{r}, \mathbf{d}) \leq 1 \quad \forall j, \forall (\mathbf{r}, \mathbf{d}) \end{aligned} \quad (6)$$

Here,  $\mathbb{E}[\cdot]$  denotes taking expectation over realization  $(\mathbf{r}, \mathbf{d})$  with distribution function  $F(\cdot)$  and  $x_j(\mathbf{r}, \mathbf{d})$  could be interpreted as the probability that the request is served using resource  $j$  by the prophet given it is revealed as  $(\mathbf{r}, \mathbf{d})$ , regardless of the time period.

**Theorem 1** *It holds that  $\text{LP}^{\text{UB}} \geq \mathbb{E}[V^{\text{off}}(\mathbf{I})]$ .*

*Proof:* We use  $\{x_j^t(\mathbf{I})\}$  to denote one optimal solution of (3) given the arriving sequence of requests  $\mathbf{I}$  and denote  $x_j^t(\mathbf{r}, \mathbf{d}) = \mathbb{E}[x_j^t(\mathbf{I}) | (\mathbf{r}^t, \mathbf{d}^t) = (\mathbf{r}, \mathbf{d})]$ . Then we have

$$0 \leq x_j^t(\mathbf{r}, \mathbf{d}) \leq 1 \quad \text{and} \quad \sum_{j=1}^m x_j^t(\mathbf{I}) \leq 1 \Rightarrow \sum_{j=1}^m x_j^t(\mathbf{r}, \mathbf{d}) \leq 1 \quad (7)$$

Also, we have that

$$\mathbb{E}[V^{\text{off}}(\mathbf{I})] = \mathbb{E}\left[\sum_{t=1}^T \sum_{j=1}^m r_j^t \cdot x_j^t(\mathbf{I})\right] = \sum_{t=1}^T \mathbb{E}\left[\mathbb{E}\left[\sum_{j=1}^m r_j^t \cdot x_j^t(\mathbf{I}) | (\mathbf{r}^t, \mathbf{d}^t) = (\mathbf{r}, \mathbf{d})\right]\right] = \sum_{t=1}^T \mathbb{E}\left[\sum_{j=1}^m r_j \cdot x_j^t(\mathbf{r}, \mathbf{d})\right] \quad (8)$$

We could further obtain the following constraint regarding  $x_j^t(\mathbf{r}, \mathbf{d})$ :

$$\sum_{t=1}^T \mathbb{E}\left[\sum_{j=1}^m d_j \cdot x_j^t(\mathbf{r}, \mathbf{d})\right] = \sum_{t=1}^T \mathbb{E}\left[\mathbb{E}\left[\sum_{j=1}^m d_j^t \cdot x_j^t(\mathbf{I}) | (\mathbf{r}^t, \mathbf{d}^t) = (\mathbf{r}, \mathbf{d})\right]\right] = \mathbb{E}\left[\sum_{t=1}^T \sum_{j=1}^m d_j^t \cdot x_j^t(\mathbf{I})\right] \leq c_j \quad \forall j \quad (9)$$

Since the request distribution is stationary across different time periods and the offline optimal solution made by the prophet is not influenced by the order of the sequence  $\mathbf{I}$ , there must exists one optimal solution of (3) such that  $x_j^{t_1}(\mathbf{r}, \mathbf{d}) = x_j^{t_2}(\mathbf{r}, \mathbf{d})$  for arbitrary  $t_1$  and  $t_2$ . Thus, we could suppress the notation  $t$  in  $x_j^t(\mathbf{r}, \mathbf{d})$ . Then given (7), (8) and (9), it holds that  $\text{LP}^{\text{UB}} \geq \mathbb{E}[V^{\text{off}}(\mathbf{I})]$ .

□

When the request distribution has a finite support, (6) is simply a finite-dimensional linear programming. When it has an infinite support, (6) is an infinite linear programming and is a special case of the general formulation studied in Hernández-Lerma and Lasserre (1998). Then, the finite-dimensional approximation scheme proposed in Hernández-Lerma and Lasserre (1998) could be directly applied to solve (6). Specifically, for any  $\varepsilon > 0$ , we could obtain a feasible solution  $\{x_j^\varepsilon(\mathbf{r}, \mathbf{d})\}$  of (6) such that  $T \cdot \mathbb{E}[\sum_{j=1}^m r_j \cdot x_j^\varepsilon(\mathbf{r}, \mathbf{d})] \geq (1 - \varepsilon) \text{LP}^{\text{UB}}$ . We will use  $\{x_j^\varepsilon(\mathbf{r}, \mathbf{d})\}$  to approximate the optimal solution of (6), denoted as  $\{x_j^*(\mathbf{r}, \mathbf{d})\}$ . Since  $\varepsilon$  could be made arbitrarily small, this approximation will not influence the competitive ratio of our policy and thus it is enough to directly deal with  $\{x_j^*(\mathbf{r}, \mathbf{d})\}$ . In what follows, we will derive our policy based on  $\{x_j^*(\mathbf{r}, \mathbf{d})\}$  and discuss the high level idea.

At each time period  $t$ , we will randomly route request  $t$  with realization  $(\mathbf{r}, \mathbf{d})$  to resource  $j$  with probability  $x_j^*(\mathbf{r}, \mathbf{d})$ . By saying routing a request to resource  $j$ , we mean that we will choose resource  $j$  as the single potential candidate to serve this request and whether or not to accept the request is decided independently by its own accept/reject rule. This random routing approach would enable us to reduce the multi-resource problem to multiple single-resource problems. We then discuss the reject/accept rule for each single-resource problem. Define random variables

$$\tilde{Y}_j(t) = \tilde{d}_j^t \cdot 1_{\{\text{request } t \text{ is routed to resource } j\}}$$

If the accept/reject rule for resource  $j$  is to accept all the requests routed to it as long as there is enough remaining capacity, then the expected reward collected from assigning resource  $j$  after the random routing procedure could be bounded naturally by

$$\begin{aligned} V_j &\geq \sum_{t=1}^T \mathbb{E}[\tilde{r}_j^t \cdot 1_{\{\tilde{Y}_j(t) > 0\}} \cdot 1_{\{\sum_{\tau=1}^t \tilde{Y}_j(\tau) \leq c_j\}}] \\ &= \sum_{t=1}^T \mathbb{E} \left[ \mathbb{E}[\tilde{r}_j^t \cdot 1_{\{\tilde{Y}_j(t) > 0\}} \cdot 1_{\{\sum_{\tau=1}^{t-1} \tilde{Y}_j(\tau) \leq c_j - y\}} | \tilde{r}_j^t = x, \tilde{Y}_j(t) = y] \right] \\ &= \sum_{t=1}^T \int_{x>0, y>0} x \cdot P\left(\sum_{\tau=1}^{t-1} \tilde{Y}_j(\tau) \leq c_j - y\right) dP(\tilde{r}_j^t = x, \tilde{Y}_j(t) = y) \\ &= \int_{x>0, y>0} x \cdot \left(\sum_{t=1}^T P\left(\sum_{\tau=1}^{t-1} \tilde{Y}_j(\tau) \leq c_j - y\right)\right) dP(\tilde{r}_j^1 = x, \tilde{Y}_j(1) = y) \end{aligned}$$

The last equality holds due to that the distribution of  $(\tilde{r}_j^t, \tilde{Y}_j(t))$  is stationary across time. Also denote  $\text{LP}_j^{\text{UB}}$  as the upper bound of the  $j$ th single-resource problem, then we have

$$\text{LP}_j^{\text{UB}} = T \cdot \mathbb{E}[r_j \cdot x_j^*(\mathbf{r}, \mathbf{d})] = T \cdot \int_{x>0, y>0} x dP(\tilde{r}_j^1 = x, \tilde{Y}_j(1) = y)$$

As long as we could find a constant  $\alpha > 0$  such that  $\sum_{t=1}^T P(\sum_{\tau=1}^{t-1} \tilde{Y}_j(\tau) \leq c_j - y) \geq \alpha \cdot T$  holds for all  $y$ , we could immediately establish that  $V_j \geq \alpha \cdot \text{LP}_j^{\text{UB}}$  and thus the competitive ratio would be



$\alpha$ . However, when the size of the accepted request could take any value among the whole interval  $(0, c_j]$ , one could not lower bound  $\sum_{t=1}^T P(\sum_{\tau=1}^{t-1} \tilde{Y}_j(\tau) \leq c_j - y)$  by  $\alpha T$  such that  $\alpha > 0$ , since  $c_j - y$  could be arbitrarily close to 0. Thus, we will specify our accept/reject rule such that the size of the accepted request is restricted to be among a sub-interval of  $(0, c_j]$ . Our accept/reject rule is described in the following.

We will allow resource  $j$  to accept either large size requests or small size requests. Specifically, when  $d_j > \frac{c_j}{2}$ , we will call the request as large size request and when  $d_j \leq \frac{c_j}{2}$ , we will call the request as small size request. Thus, the size of the accepted request is restricted to be either among  $(0, \frac{c_j}{2}]$  or  $(\frac{c_j}{2}, c_j]$ . We could show that for resource  $j$ , the expected reward obtained from only accepting large size requests is at least  $g^1(u_j) \cdot l_j$  and the expected reward obtained from only accepting small size requests is at least  $g^2(u_j) \cdot s_j$ , where

$$l_j = T \cdot \mathbb{E}[r_j \cdot x_j^*(\mathbf{r}, \mathbf{d}) \cdot \mathbf{1}_{\{d_j > \frac{c_j}{2}\}}], \quad s_j = T \cdot \mathbb{E}[r_j \cdot x_j^*(\mathbf{r}, \mathbf{d}) \cdot \mathbf{1}_{\{d_j \leq \frac{c_j}{2}\}}], \quad u_j = T \cdot \mathbb{E}[d_j \cdot x_j^*(\mathbf{r}, \mathbf{d}) \cdot \mathbf{1}_{\{d_j > \frac{c_j}{2}\}}] \quad (10)$$

and

$$g^1(u_j) = \frac{c_j}{2u_j} \cdot (1 - e^{-\frac{2u_j}{c_j}}), \quad g^2(u_j) = \frac{c_j}{2(c_j - u_j)} \cdot (1 - e^{-\frac{2(c_j - u_j)}{c_j}}) \quad (11)$$

It is obvious that if  $g^1(u_j) \cdot l_j \geq g^2(u_j) \cdot s_j$  (resp.  $g^1(u_j) \cdot l_j < g^2(u_j) \cdot s_j$ ), it is more beneficial for resource  $j$  to only accept large (resp. small) size requests. Thus we classify all the resources into two sets:

$$L = \{j : g^1(u_j) \cdot l_j \geq g^2(u_j) \cdot s_j\} \quad \text{and} \quad S = \{j : g^1(u_j) \cdot l_j < g^2(u_j) \cdot s_j\} \quad (12)$$

and resources in  $L$  (resp.  $S$ ) will be allowed to only accept large (resp. small) size requests. Our algorithm is formally described in Algorithm 1. In what follows, we will analyze the performance

---

**Algorithm 1** Nonadaptive Threshold Policy (NTP)

---

- 1: Obtain optimal solution  $\{x_j^*(\mathbf{r}, \mathbf{d})\}$  by solving (6).
  - 2: Classify all the resources into two sets  $L$  and  $S$  according to (12).
  - 3: At time period  $t = 1, 2, \dots, T$ , do the following:
  - 4: Route the request  $t$  with realization  $(\mathbf{r}, \mathbf{d})$  to resource  $j$  with probability  $x_j^*(\mathbf{r}, \mathbf{d})$ .
    - (i) If  $d_j \leq \frac{c_j}{2}$ , then accept the request if and only if  $j \in S$  and  $d_j$  does not exceed the remaining capacity of resource  $j$ .
    - (ii) If  $d_j > \frac{c_j}{2}$ , then accept the request if and only if  $j \in L$  and  $d_j$  does not exceed the remaining capacity of resource  $j$ .
- 

of Algorithm 1.

**Theorem 2** *Algorithm 1 has a competitive ratio of 0.302.*

*Proof:* Under Algorithm 1, we define the following random variables

$$\tilde{Y}_j^S(t) = \tilde{d}_j^t \cdot 1_{\{\text{request } t \text{ is routed to resource } j\}} \cdot 1_{\{\tilde{d}_j^t \leq \frac{c_j}{2}\}}$$

and

$$\tilde{Y}_j^L(t) = \tilde{d}_j^t \cdot 1_{\{\text{request } t \text{ is routed to resource } j\}} \cdot 1_{\{\tilde{d}_j^t > \frac{c_j}{2}\}}$$

It is obvious that  $\mathbb{E}[\tilde{Y}_j^S(t)] = \mathbb{E}[d_j \cdot x_j^*(\mathbf{r}, \mathbf{d}) \cdot 1_{\{d_j \leq \frac{c_j}{2}\}}]$  and  $\mathbb{E}[\tilde{Y}_j^L(t)] = \mathbb{E}[d_j \cdot x_j^*(\mathbf{r}, \mathbf{d}) \cdot 1_{\{d_j > \frac{c_j}{2}\}}] = \frac{u_j}{T}$ .

Note that

$$\mathbb{E}[d_j \cdot x_j^*(\mathbf{r}, \mathbf{d}) \cdot 1_{\{d_j \leq \frac{c_j}{2}\}}] + \mathbb{E}[d_j \cdot x_j^*(\mathbf{r}, \mathbf{d}) \cdot 1_{\{d_j > \frac{c_j}{2}\}}] = \mathbb{E}[d_j \cdot x_j^*(\mathbf{r}, \mathbf{d})] \leq \frac{c_j}{T}$$

we have

$$\mathbb{E}[\tilde{Y}_j^S(t)] \leq \frac{c_j - u_j}{T} \quad (13)$$

Also, we have for each  $t$

$$\begin{aligned} \frac{s_j}{T} &= \mathbb{E}[r_j \cdot x_j^*(\mathbf{r}, \mathbf{d}) \cdot 1_{\{d_j \leq \frac{c_j}{2}\}}] = \mathbb{E}[\tilde{r}_j^t \cdot 1_{\{\text{request } t \text{ is routed to resource } j\}} \cdot 1_{\{\tilde{d}_j^t \leq \frac{c_j}{2}\}}] \\ &= \int_{x>0, y>0} x dP(\tilde{r}_j^t = x, \tilde{Y}_j^S(t) = y) \end{aligned} \quad (14)$$

where the last equality holds due to that the event that  $\tilde{Y}_j^S(t) > 0$  is equivalent to the event that  $1_{\{\text{request } t \text{ is routed to resource } j\}} \cdot 1_{\{\tilde{d}_j^t \leq \frac{c_j}{2}\}} = 1$ . Similarly, we have

$$\frac{l_j}{T} = \int_{x>0, y>0} x dP(\tilde{r}_j^t = x, \tilde{Y}_j^L(t) = y) \quad (15)$$

For each resource  $j$ , let  $V_j^{\text{NTP}}(\mathbf{I})$  denotes the expected reward collected from assigning resource  $j$  by Algorithm 1, then we consider the following two situations:

(i). When  $j \in L$ , request  $t$  is accepted by resource  $j$  if and only if  $\tilde{Y}_j^L(t) > 0$  and resource  $j$  hasn't been assigned yet, i.e., for all  $\tau < t$ ,  $\tilde{Y}_j^L(\tau) = 0$ . Thus, we must have

$$\begin{aligned} \mathbb{E}[V_j^{\text{NTP}}(\mathbf{I})] &= \sum_{t=1}^T \mathbb{E}[\tilde{r}_j^t \cdot 1_{\{\tilde{Y}_j^L(t) > 0\}} \cdot 1_{\{\tilde{Y}_j^L(\tau) = 0, \tau=1,2,\dots,t-1\}}] \\ &= \sum_{t=1}^T \int_{x>0, y>0} x \cdot \left( \prod_{\tau=1}^{t-1} P(\tilde{Y}_j^L(\tau) = 0) \right) dP(\tilde{r}_j^t = x, \tilde{Y}_j^L(t) = y) \\ &= \sum_{t=1}^T \prod_{\tau=1}^{t-1} P(\tilde{Y}_j^L(\tau) = 0) \cdot \int_{x>0, y>0} x dP(\tilde{r}_j^t = x, \tilde{Y}_j^L(t) = y) \\ &= \sum_{t=1}^T \prod_{\tau=1}^{t-1} P(\tilde{Y}_j^L(\tau) = 0) \cdot \frac{l_j}{T} \end{aligned}$$

where the last equality holds due to (15). Moreover, notice that  $\tilde{Y}_j^L(t) > 0$  implies  $\tilde{Y}_j^L(t) > \frac{c_j}{2}$ , we have

$$\frac{c_j}{2} \cdot P(\tilde{Y}_j^L(t) > 0) \leq \mathbb{E}[\tilde{Y}_j^L(t)] = \frac{u_j}{T}$$

which implies that  $P(\tilde{Y}_j^L(t) > 0) \leq \frac{2u_j}{c_j T}$ . Then we have

$$\sum_{t=1}^T \prod_{\tau=1}^{t-1} (1 - P(\tilde{Y}_j^L(\tau) > 0)) \geq \sum_{t=1}^T (1 - \frac{2u_j}{c_j T})^{t-1} = \frac{c_j T}{2u_j} \cdot (1 - (1 - \frac{2u_j}{c_j T})^T) \geq g^1(u_j) \cdot T$$

Thus, notice that  $g^1(u_j) \cdot l_j \geq g^2(u_j) \cdot s_j$ , we have that

$$\frac{\mathbb{E}[V_j^{\text{NTP}}(\mathbf{I})]}{s_j + l_j} \geq \frac{g^1(u_j) \cdot l_j}{s_j + l_j} \geq \frac{g^1(u_j) \cdot g^2(u_j)}{g^1(u_j) + g^2(u_j)}$$

(ii). When  $j \in S$ , request  $t$  is served by resource  $j$  if  $\tilde{Y}_j^S(t) > 0$  and  $\sum_{\tau=1}^t \tilde{Y}_j^S(\tau) \leq c_j$ . Thus, we have

$$\begin{aligned} \mathbb{E}[V_j^{\text{NTP}}(\mathbf{I})] &\geq \sum_{t=1}^T \mathbb{E}[\tilde{r}_j^t \cdot 1_{\{\tilde{Y}_j^S(t) > 0\}} \cdot 1_{\{\sum_{\tau=1}^t \tilde{Y}_j^S(\tau) \leq c_j\}}] \\ &= \sum_{t=1}^T \mathbb{E} \left[ \mathbb{E}[\tilde{r}_j^t \cdot 1_{\{\tilde{Y}_j^S(t) > 0\}} \cdot 1_{\{\sum_{\tau=1}^{t-1} \tilde{Y}_j^S(\tau) \leq c_j - y\}} | \tilde{r}_j^t = x, \tilde{Y}_j^S(t) = y] \right] \\ &= \sum_{t=1}^T \int_{x>0, y>0} x \cdot P(\sum_{\tau=1}^{t-1} \tilde{Y}_j^S(\tau) \leq c_j - y) dP(\tilde{r}_j^t = x, \tilde{Y}_j^S(t) = y) \\ &= \int_{x>0, y>0} x \cdot (\sum_{t=1}^T P(\sum_{\tau=1}^{t-1} \tilde{Y}_j^S(\tau) \leq c_j - y)) dP(\tilde{r}_j^1 = x, \tilde{Y}_j^S(1) = y) \end{aligned} \quad (16)$$

The last equality holds due to that the distribution of  $(\tilde{r}_j^t, \tilde{Y}_j^S(t))$  is stationary across  $t$ . Since  $\tilde{Y}_j^S(1) \in [0, \frac{c_j}{2}]$ ,  $y$  is restricted to take value only among  $(0, \frac{c_j}{2}]$ , then we have the following bound.

**Claim 1** Suppose for each  $t$ ,  $Y_j^t$  are nonnegative independent random variables with mean  $E[Y_j^t] \leq \frac{c_j - u_j}{T}$ , then for each  $y \in (0, \frac{c_j}{2}]$ , we have that

$$\sum_{t=1}^T P(\sum_{\tau=1}^{t-1} Y_j^\tau \leq c_j - y) \geq \sum_{t=1}^T P(\sum_{\tau=1}^{t-1} Y_j^\tau \leq \frac{c_j}{2}) \geq \frac{T}{2} \cdot \frac{c_j}{c_j - u_j} \cdot (1 - e^{-\frac{2(c_j - u_j)}{c_j}}) = T \cdot g^2(u_j) \quad (17)$$

The proof is relegated to the appendix. Then, from (14), we have that

$$\mathbb{E}[V_j^{\text{NTP}}(\mathbf{I})] \geq g^2(u_j) \cdot s_j$$

Notice that  $g^2(u_j) \cdot s_j \geq g^1(u_j) \cdot l_j$ , we have

$$\frac{\mathbb{E}[V_j^{\text{NTP}}(\mathbf{I})]}{s_j + l_j} \geq \frac{g^1(u_j) \cdot g^2(u_j)}{g^1(u_j) + g^2(u_j)}$$

Thus, in both cases, we establish the following result:

$$\frac{\mathbb{E}[V_j^{\text{NTP}}(\mathbf{I})]}{s_j + l_j} \geq \frac{g^1(u_j) \cdot g^2(u_j)}{g^1(u_j) + g^2(u_j)} \geq \min_{0 \leq u_j \leq c_j} \frac{g^1(u_j) \cdot g^2(u_j)}{g^1(u_j) + g^2(u_j)} = \frac{1 - e^{-2}}{3 - e^{-2}} \approx 0.302 \quad (18)$$

The detailed procedure of solving the single-variable minimization problem in (18) is shown in the appendix. Our proof is immediately completed by noting that  $LP^{UB} = \sum_{j=1}^m (s_j + l_j) \geq \mathbb{E}[V^{\text{off}}(\mathbf{I})]$  and  $\mathbb{E}[V^{\text{NTP}}(\mathbf{I})] = \sum_{j=1}^m \mathbb{E}[V_j^{\text{NTP}}(\mathbf{I})]$ .  $\square$

Moreover, we could show that there does not exist an online algorithm with a competitive ratio larger than 0.5 even for the single-resource setting by constructing a problem instance in the following theorem. Note that a 0.5 upper bound of the competitive ratio is also proved in Stein et al. (2019) where the reward of each request is assumed to be equal to the size, however, they assumed the requests arrive according to a non-homogeneous Poisson process and their problem instance is built on the non-homogeneous property of the arrival process. In contrast, we proved the 0.5 upper bound when the reward and the size can be arbitrarily different but the arrival process is time homogeneous.

**Theorem 3** *The competitive ratio of any online algorithm is upper bounded by 0.5 even for the single-resource setting.*

*Proof:* Consider a single resource case with an initial capacity 1. We use  $\mathbf{I}$  to denote the sample path of the arrival of  $T$  requests and we assume that for each  $t$ , the distribution of  $(\tilde{r}^t, \tilde{d}^t)$  is a two point distribution that

$$P((\tilde{r}^t, \tilde{d}^t) = (r_1, d_1)) = 1 - \varepsilon \quad \text{and} \quad P((\tilde{r}^t, \tilde{d}^t) = (r_2, d_2)) = \varepsilon$$

where  $r_1 = 1$ ,  $d_1 = \frac{1}{T}$ ,  $r_2 = \frac{T \cdot r_1 \cdot \beta}{1 - \beta}$ ,  $d_2 = 1$  and  $\varepsilon$  is a constant satisfying  $(1 - \varepsilon)^T = \beta$ . Here,  $\beta$  is a constant to be determined later and we assume that  $\beta \in (0.5, 1)$ . Then, it holds that  $r_2 \geq Tr_1$  and the prophet will choose to serve the request with realization  $(r_2, d_2)$  as long as it appears. Thus we have that

$$\mathbb{E}[V^{\text{off}}(\mathbf{I})] = Tr_1(1 - \varepsilon)^T + (1 - (1 - \varepsilon)^T)r_2 = 2\beta Tr_1$$

Moreover, notice that once a request with realization  $(r_1, d_1)$  is served, there will not be enough capacity to serve any request with realization  $(r_2, d_2)$ . Thus the decision of the online algorithm is to decide a  $1 \leq k \leq T$  such that requests with realization  $(r_1, d_1)$  could only be accepted after the first  $k - 1$  time periods. Then its expected reward would be

$$\mathbb{E}[V^k(\mathbf{I})] = (1 - (1 - \varepsilon)^k)r_2 + (1 - \varepsilon)^k \cdot [r_1 + (T - k)(1 - \varepsilon)r_1] \quad (19)$$

Next, we will show that  $\mathbb{E}[V^k(\mathbf{I})] \geq \mathbb{E}[V^{k+1}(\mathbf{I})]$  holds for every  $1 \leq k \leq T - 1$ , thus  $k = 1$  is the optimal choice for the online algorithm. Notice that from (19), we have the following equivalent expression of  $\mathbb{E}[V^k(\mathbf{I})] \geq \mathbb{E}[V^{k+1}(\mathbf{I})]$ :

$$\mathbb{E}[V^k(\mathbf{I})] \geq \mathbb{E}[V^{k+1}(\mathbf{I})] \Leftrightarrow (\varepsilon - \varepsilon^2)k \leq 1 - \varepsilon - \frac{\varepsilon\beta T}{1 - \beta} + (\varepsilon - \varepsilon^2)T \quad (20)$$

It is enough to show that (20) holds for  $k = T - 1$ . Notice that from the definition, we have  $\varepsilon = \frac{1}{T} \cdot \log \frac{1}{\beta} + o(\frac{1}{T})$ . Then substituting it into (20) for  $k = T - 1$ , we derive the following equivalent expression of (20) by neglecting the  $o(1)$  term:

$$(\varepsilon - \varepsilon^2)(T - 1) \leq 1 - \varepsilon - \frac{\varepsilon\beta T}{1 - \beta} + (\varepsilon - \varepsilon^2)T \Leftrightarrow \frac{\beta}{1 - \beta} \cdot \log \frac{1}{\beta} \leq 1 \quad (21)$$

It is easy to check that (21) holds for  $0.5 < \beta < 1$ , thus we have proved that  $k = 1$  is optimal for the online algorithm. Also, notice that

$$\mathbb{E}[V^1(\mathbf{I})] = T \cdot r_1 + O(1)$$

the optimal competitive ratio is  $\frac{1}{2\beta}$ , which converges to 0.5 as  $\beta \rightarrow 1$ .  $\square$

#### 4. Regret Bound for Finite-Support Reward Case

In this section, we will consider our online resource allocation problem under the setting that the reward distribution has a finite support. Specifically, we will make the following assumption:

**Assumption 2** *For each  $t$ , the value of  $\tilde{\mathbf{r}}^t$  is drawn independently from a finite set  $\{\mathbf{r}_1, \mathbf{r}_2, \dots, \mathbf{r}_n\}$ , where  $\mathbf{r}_i = [r_{i1}, r_{i2}, \dots, r_{im}]$ . Moreover, given that  $\tilde{\mathbf{r}}^t = \mathbf{r}_i$ , we have  $\tilde{\mathbf{d}}^t = \mathbf{b}_i \cdot \tilde{u}_i^t$ , where  $\mathbf{b}_i = [b_{i1}, b_{i2}, \dots, b_{im}]$  denotes the positive deterministic weight and  $\tilde{u}_i^t$  is a single-dimensional random variable.*

In what follows, for each  $t$ , we will use  $p_i$  to denote the probability that  $\tilde{\mathbf{r}}^t = \mathbf{r}_i$  and use  $F_i(\cdot)$  to denote the distribution of the random variable  $\tilde{u}_i^t$  given that  $\tilde{\mathbf{r}}^t = \mathbf{r}_i$ , where the realization of  $\tilde{u}_i^t$  will be denoted as  $u_i^t$ . We only focus on the case where  $F_i(\cdot)$  is continuous for each  $i$ .

Indeed, under Assumption 2, we can show that the linear programming prophet upper bound (6) could be reduced into  $n$  sub-LPs and accordingly, our original online resource allocation problem could be reduced to  $n$  separate sub-problems, where in each sub-problem the reward of the request is deterministic and each sub-LP serves as the prophet upper bound for each sub-problem. We further show that the optimal solution of each sub-LP possesses a threshold structure and the thresholds could be given in a closed-form expression. Then, based on this threshold structure, together with some mild regularity conditions on the distribution functions  $\{F_i(\cdot), i = 1, 2, \dots, n\}$ , we could show a convex structure of the thresholds and then obtain a second-order upper estimates of how the optimal value of each sub-LP would vary over the right hand side (RHS) of the constraints. By applying a re-solving policy in each sub-problem, we show in our regret analysis that the first order terms in the estimate will cancel out and only the second order terms will be left, which will finally lead to a  $O(\log T)$  regret bound.

#### 4.1. Prophet Upper Bound

In this subsection, we first show how to reduce (6) into  $n$  sub-LPs and then characterize the optimal solution of each sub-LP in a closed-form expression. We consider the sub-LP of the following formulation:

$$\begin{aligned}
 G_i(\tilde{\mathbf{c}}_i, t) := & \max \quad (T - t + 1) \cdot p_i \cdot \mathbb{E}_i \left[ \sum_{j=1}^m r_{ij} \cdot x_{ij}(u) \right] \\
 \text{s.t.} \quad & (T - t + 1) \cdot p_i \cdot b_{ij} \cdot \mathbb{E}_i[u \cdot x_{ij}(u)] \leq \tilde{c}_{ij} \quad \forall j \\
 & \sum_{j=1}^m x_{ij}(u) \leq 1 \quad \forall u \\
 & 0 \leq x_{ij}(u) \leq 1 \quad \forall j, \forall u
 \end{aligned} \tag{22}$$

where  $\tilde{\mathbf{c}}_i = [\tilde{c}_{i1}, \tilde{c}_{i2}, \dots, \tilde{c}_{im}]$  and  $\mathbb{E}_i[\cdot]$  denotes taking expectation over the realization  $u$  with distribution function  $F_i(\cdot)$ .

**Lemma 1** *It holds that*

$$\begin{aligned}
 LP^{UB} = & \max \quad \sum_{i=1}^n G_i(\tilde{\mathbf{c}}_i, 1) \\
 \text{s.t.} \quad & \sum_{i=1}^n \tilde{c}_{ij} \leq c_j \quad \forall j \\
 & \tilde{c}_{ij} \geq 0 \quad \forall i, \forall j
 \end{aligned} \tag{23}$$

We then characterize the optimal solution of the sub-LP (22) and show the threshold structure. Specifically, for each  $i$ , denote  $\{i_1, i_2, \dots, i_m\}$  as a permutation of  $\{1, 2, \dots, m\}$  such that  $r_{ii_1} \geq r_{ii_2} \geq \dots \geq r_{ii_m} \geq 0$  and we set  $r_{ii_{m+1}} = 0$ , then for each  $i, j, t$ , we define the threshold  $\mu_t^{ij}(\tilde{\mathbf{c}}_i)$  as the solution of the following equation:

$$p_i \cdot \int_0^{\mu_t^{ij}(\tilde{\mathbf{c}}_i)} u dF_i(u) = \frac{\sum_{k=1}^j \tilde{c}_{ii_k} / b_{ii_k}}{T - t + 1} \tag{24}$$

If there is no  $\mu_t^{ij}(\tilde{\mathbf{c}}_i)$  satisfying the above equation, we set  $\mu_t^{ij}(\tilde{\mathbf{c}}_i) = \infty$ .

**Lemma 2** *For each  $i, j, u$ , define the solution  $\hat{x}_{ii_j}(u)$  by*

$$\hat{x}_{ii_j}(u) = \begin{cases} 1, & \text{if } \mu_t^{ii_{j-1}}(\tilde{\mathbf{c}}_i) < u \leq \mu_t^{ii_j}(\tilde{\mathbf{c}}_i) \\ 0, & \text{otherwise} \end{cases} \tag{25}$$

where  $\mu_t^{ii_0}(\tilde{\mathbf{c}}_i)$  is set to be 0. Then  $\{\hat{x}_{ii_j}(u)\}$  is an optimal solution to (22) and it holds that

$$G_i(\tilde{\mathbf{c}}_i, t) = (T - t + 1) \cdot p_i \cdot \sum_{j=1}^m (r_{ii_j} - r_{ii_{j+1}}) \cdot F_i(\mu_t^{ii_j}(\tilde{\mathbf{c}}_i)) \tag{26}$$

Together, Lemma 1 and Lemma 2 will provide a closed-form characterization of the optimal solution of the linear programming prophet upper bound (6). Indeed, notice that  $G_i(\tilde{\mathbf{c}}_i, t)$  is a concave function over  $\tilde{\mathbf{c}}_i$ , the optimization problem (23) is a convex optimization problem, and we could use the following formula to obtain the supergradient of  $G_i(\tilde{\mathbf{c}}_i, t)$  immediately:

$$\frac{\partial G_i(\tilde{\mathbf{c}}_i, t)}{\partial \tilde{c}_{ij}} = \sum_{k=j}^m \frac{r_{ii_k} - r_{ii_{k+1}}}{b_{ii_j} \cdot \mu_t^{ii_k}(\tilde{\mathbf{c}}_i)}, \quad \forall j$$

Thus, the optimization problem (23) is tractable and could be solved efficiently.

**Remark:** when there is only one resource and the reward is unitary, i.e.,  $m = n = 1$ , our prophet upper bound (6) is identical to the upper bound in Arlotto and Xie (2020). However, their approach to derive the prophet upper bound is based on an observation that when there is only one resource and the reward is unitary, the hindsight optimal policy is to simply serve the requests in an increasing order of the size. Thus, the order statistics of the size of the requests is enough to characterize the hindsight optimum. Their approach could not be directly applied to a more general setting where this observation doesn't hold. Specifically, when there are multiple resources and the reward could take multiple values, the hindsight optimum is an integer programming (3), the solution of which should not be serving the request from the smallest size. Instead, our approach is based on directly dealing with the linear programming prophet upper bound (6) and show its specific threshold structure.

## 4.2. Regularity Conditions

In this subsection, we will describe the regularity conditions that the distribution functions  $F_i(\cdot)$  need to satisfy. A special case of our problem where there is only one resource and the reward is unitary is identical to the dynamic and stochastic knapsack problem with equal reward studied in a stream of literature: Coffman et al. (1987), Bruss and Robertson (1991), Papastavrou et al. (1996), Arlotto and Xie (2020). All these papers assumed some regularity conditions on the distribution functions to obtain their results. One may see the necessity of the regularity conditions by referring to Section 5 in Papastavrou et al. (1996) which shows that one could not expect some structural properties such as the monotonicity of the optimal threshold and the concavity of the optimal value for general distributions. Specifically, Arlotto and Xie (2020) proved a  $O(\log T)$  regret bound for this knapsack problem by assuming the distribution function belongs to the so-called *typical class*. In what follows, we adopt the *typical class* conditions with only one minor change which will be discussed later.

**Assumption 3** For some  $\bar{\omega} > 0$  and for all  $i$ , the distribution function  $F_i(\cdot)$  has a continuous density function  $f_i(\cdot)$  and satisfies the following two conditions:

1. (*Behavior at Zero*) There exists a constant  $0 < \lambda < 1$  and two constants  $1 < \gamma_1 < \gamma_2$  such that

$$\gamma_1 \cdot F_i(\lambda w) \leq F_i(w) \leq \gamma_2 \cdot F_i(\lambda w) \quad \text{for all } w \in (0, \bar{\omega}) \quad (27)$$

2. (*Monotonicity*) The function  $w \mapsto w^3 f_i(w)$  is a non-decreasing function over  $(0, \bar{\omega})$ .

The only difference between our Assumption 3 and the *typical class* conditions in Arlotto and Xie (2020) lies in condition 1. *Typical class* only assumed  $F_i(w)$  to be lower bounded by  $F_i(\lambda w)$ , i.e., they only assumed  $\gamma_1 \cdot F_i(\lambda w) \leq F_i(w)$ , while in our assumption, we assume  $F_i(w)$  to be both lower bounded and upper bounded by  $F_i(\lambda w)$ . The discussions in Section 5 of Arlotto and Xie (2020) showed that their *typical class* conditions could cover a very broad class of continuous distributions. Moreover, it is easy to check that the following distributions they have considered continue to satisfy both conditions in Assumption 3:

1. Uniform distribution, exponential distribution and logit-normal distribution.
2. Truncated normal distribution on  $(0, b)$  and truncated logistic distribution on  $(0, b)$ .
3. Power distribution with distribution function  $F(x) = Ax^\alpha$  for  $A, \alpha > 0$  truncated on  $(0, b)$ .
4. Distributions with convex distribution function  $F(\cdot)$  and continuous density function  $f(\cdot)$  such that  $f(0) > 0$ .
5. The mixture distribution of some distributions satisfying both conditions in Assumption 3.

We show in the next lemma that condition 1 in Assumption 3 will enable us to derive the following estimate over the distribution functions  $F_i(\cdot)$ .

**Lemma 3** *If there exists a continuous distribution  $F(\cdot)$  such that for some  $\bar{\omega} > 0$ , Condition 1 in Assumption 3 is satisfied, i.e., there exists a constant  $0 < \lambda < 1$  and two constants  $1 < \gamma_1 < \gamma_2$  such that*

$$\gamma_1 \cdot F(\lambda w) \leq F(w) \leq \gamma_2 \cdot F(\lambda w) \quad \text{for all } w \in (0, \bar{\omega}) \quad (28)$$

*then there exists a constant  $M > 1$  such that for any  $w_1, w_2$  satisfying  $0 < w_1 < w_2 < \bar{\omega}$ , we have*

$$\frac{w_2(F(w_2) - F(w_1))}{\int_{w_1}^{w_2} w dF(w)} \leq M \quad (29)$$

Also, we could obtain the following convex property regarding the threshold  $\mu_t^{ij}(\tilde{\mathbf{c}}_i)$  for each  $i$  and  $j$  under condition 2 in Assumption 3.

**Lemma 4** *Suppose Assumption 3 holds, then for each  $i, j$ , and any  $k = 1, 2, \dots, j$ , the function*

*$\frac{1}{\mu_t^{ij}(\tilde{\mathbf{c}}_i)}$  is a convex function over  $\tilde{\mathbf{c}}_{ii_k}$ .*



The proofs of the above two lemmas are relegated to the appendix. Together, Lemma 3 and Lemma 4 would enable us to obtain the second-order upper estimate of the sensitivity of  $G_i(\tilde{\mathbf{c}}_i, t)$  over  $\tilde{\mathbf{c}}_i$ . Indeed, given the formulation of  $G_i(\tilde{\mathbf{c}}_i, t)$  in (26), it is enough to consider the sensitivity of  $F_i(\mu_t^{ii_j}(\tilde{\mathbf{c}}_i))$  over  $\tilde{\mathbf{c}}_i$  for each  $j$ . The following second-order estimate generalizes the estimate in Arlotto and Xie (2020) from the single-resource setting to the multi-resource setting and the proof could be found in the appendix.

**Lemma 5** *Suppose Assumption 3 holds, then for each  $i, j$  and any  $k = 1, 2, \dots, j$ , we have that*

$$F_i(\mu_t^{ii_j}(\tilde{\mathbf{c}}_i)) - F_i(\mu_t^{ii_j}(\tilde{\mathbf{c}}_i - b_{ii_k} u \cdot \mathbf{e}_{i_k})) \leq \frac{(M-1) \cdot u^2}{(\tilde{c}_{ii_k}/b_{ii_k})p_i(T-t+1)\mu_t^{ii_j}(\tilde{\mathbf{c}}_i)} + \frac{u}{p_i(T-t+1)\mu_t^{ii_j}(\tilde{\mathbf{c}}_i)} \quad (30)$$

holds for any  $u \in [0, \tilde{c}_{ii_k}/b_{ii_k}]$ .

### 4.3. Adaptive Threshold Policy

We now introduce our adaptive threshold policy and prove the corresponding regret bound. Since the optimal solution and the sensitivity of each sub-LP (22) could be fully characterized in (25) and in (30), we will reduce the original online resource allocation problem into  $n$  sub-problems to utilize this characterization. Specifically, we will divide each resource  $j$  into  $n$  parts and assign a capacity  $c_{ij}^*$  to each  $i$ th part of resource  $j$ , where  $\{c_{ij}^*\}$  is denoted as the optimal solution of (23). Then, for each request with a realized reward  $\mathbf{r}_i$ , we will only consider using the  $i$ th part of each resource to serve it. By doing so, the  $i$ th sub-problem is only concerned about serving request with a deterministic reward  $\mathbf{r}_i$  using a separate part of each resource. Thus, each sub-problem will be independent from each other and it is enough to focus on each sub-problem separately.

For  $i$ th sub-problem, we will construct our control policy based on re-solving (22). Specifically, at each time period  $t$ , denote the remaining capacity of the  $i$ th part of resource  $j$  as  $c_{ij}^t$  and denote  $\mathbf{c}_i^t = [c_{i1}^t, c_{i2}^t, \dots, c_{im}^t]$ , then given  $\tilde{\mathbf{r}}^t = \mathbf{r}_i$ , the threshold structure of the optimal solution of  $G_i(\mathbf{c}_i^t, t)$  in (25) implies us to assign resource  $i_j$  to serve the request as long as  $\mu_t^{ii_{j-1}}(\mathbf{c}_i^t) < u_i^t \leq \mu_t^{ii_j}(\mathbf{c}_i^t)$ . However, the actual threshold will be truncated by the remaining capacity  $\mathbf{c}_i^t$ . Thus, in our adaptive threshold policy, we will compare  $u_i^t$  sequentially to the truncated thresholds  $h_t^{ii_j}(\mathbf{c}_i^t) = \min\{\mu_t^{ii_j}(\mathbf{c}_i^t), c_{ii_j}^t/b_{ii_j}\}$  from  $j = 1$  to  $m$  and assign resource  $i_j$  to serve the request once  $u_i^t \leq h_t^{ii_j}(\mathbf{c}_i^t)$ . Our adaptive threshold policy is formally presented in Algorithm 2.

Next, we discuss the performance of our adaptive threshold policy. For each  $i$ , denote  $V_i^{\text{ATP}_1}(\mathbf{I})$  as the total reward collected by Algorithm 2 for the  $i$ th sub-problem, i.e., the total reward collected from serving the requests with a realized reward  $\mathbf{r}_i$ , then we have

$$\mathbb{E}[V^{\text{ATP}_1}(\mathbf{I})] = \sum_{i=1}^n \mathbb{E}[V_i^{\text{ATP}_1}(\mathbf{I})] \quad (31)$$

**Algorithm 2** Adaptive Threshold Policy (ATP<sub>1</sub>)

- 
- 1: Solve (23) and denote the optimal solution as  $\{\mathbf{c}_i^*\}$ .
  - 2: At time period  $t = 1, 2, \dots, T$ :
  - 3: After request  $t$  arrives and reveals itself as  $(\mathbf{r}_i, \mathbf{b}_i \cdot u_i^t)$ , compute the thresholds  $\mu_t^{ij}(\mathbf{c}_i^t)$  for each  $j$  according to (25).
  - 4: For each  $j$ , define the truncated threshold  $h_t^{ij}(\mathbf{c}_i^t) = \min\{c_{ii_j}^t/b_{ii_j}, \mu_t^{ij}(\mathbf{c}_i^t)\}$  and then do the following:
    - (i) Compare  $u_i^t$  to the truncated thresholds  $h_t^{i1}(\mathbf{c}_i^t), h_t^{i2}(\mathbf{c}_i^t), \dots, h_t^{im}(\mathbf{c}_i^t)$  sequentially and assign the first resource  $i_j$  to serve request  $t$  such that  $u_i^t \leq h_t^{ij}(\mathbf{c}_i^t)$ . Then set  $c_{ii_j}^{t+1} = c_{ii_j}^t - b_{ii_j} \cdot u_i^t$  and set  $c_{i'j'}^{t+1} = c_{i'j'}^t$  for all other  $(i', j')$  such that  $(i', j') \neq (i, i_j)$ .
    - (ii) Reject request  $t$  if for all  $j$ ,  $u_i^t > h_t^{ij}(\mathbf{c}_i^t)$  and then set  $c_{i'j'}^{t+1} = c_{i'j'}^t$  for each  $i'$  and  $j'$ .
- 

Thus, from (23), the regret of Algorithm 2 could be expressed as the summation of the regret of each sub-problem:

$$\text{Regret}(\text{ATP}_1) \leq \sum_{i=1}^n G_i(\mathbf{c}_i^*, 1) - \mathbb{E}[V_i^{\text{ATP}_1}(\mathbf{I})] \quad (32)$$

where  $\{\mathbf{c}_i^*\}$  denotes the optimal solution of (23). For each  $i$ , we have the following upper bound of the term  $G_i(\mathbf{c}_i^*, 1) - \mathbb{E}[V_i^{\text{ATP}_1}(\mathbf{I})]$ .

**Lemma 6** Suppose Assumption 3 holds and let  $K_i$  be a constant defined as follows:

$$K_i = \left\lceil \frac{\sum_{j=1}^m c_{ii_j}^*/b_{ii_j}}{p_i \cdot \int_0^{\bar{\omega}} w dF_i(w)} \right\rceil \quad (33)$$

Then, we have the following bound:

$$G_i(\mathbf{c}_i^*, 1) - \mathbb{E}[V_i^{\text{ATP}_1}(\mathbf{I})] \leq \sum_{j=1}^m r_{ii_j} [(j+1)M - j](\log T + 1) + r_{\max}^i \cdot K_i = O(m^2 \log T) \quad (34)$$

where  $r_{\max}^i = \max\{r_{i1}, r_{i2}, \dots, r_{im}\}$  and  $M$  is the constant defined in Lemma 3.

The proof of Lemma 6 is based on first deriving the recursion of the "to-go" expected reward of the policy given the current time period  $t$  and the remaining capacity  $\mathbf{c}_i^t$ , denoted as  $V_t(\mathbf{c}_i^t)$ , in the following way:

$$V_t(\mathbf{c}_i^t) = (1 - p_i \cdot F(h_t^{ijw}(\mathbf{c}_i^t))) \cdot V_{t+1}(\mathbf{c}_i^t) + p_i \cdot \sum_{w=1}^W \int_{h_t^{ijw-1}(\mathbf{c}_i^t)}^{h_t^{ijw}(\mathbf{c}_i^t)} \{r_{jw} + V_{t+1}(\mathbf{c}_i^t - b_{ijw} u \cdot \mathbf{e}_{jw})\} dF_i(u)$$

where  $\{h_t^{ijw}(\mathbf{c}_i^t)\}$  denotes the monotone increasing subsequence of  $\{h_t^{ij}(\mathbf{c}_i^t)\}$ . Note that although the thresholds  $\{\mu_t^{ij}(\mathbf{c}_i^t)\}$  is monotone increasing in  $j$ , the actual thresholds  $\{h_t^{ij}(\mathbf{c}_i^t)\}$  involved in our policy may not be monotone due to the truncation of the remaining capacity, thus, only the

monotone subsequence  $\{h_t^{ijw}(\mathbf{c}_i^t)\}$  will show up in the above recursion. Then denoting  $\rho_t(\mathbf{c}_i^t) = G_i(\mathbf{c}_i^t, t) - V_t(\mathbf{c}_i^t)$ , we could substitute  $\rho_t(\mathbf{c}_i^t)$  into the above formula and obtain a recursion over  $\rho_t(\mathbf{c}_i^t)$ . We will use the second-order upper estimate in Lemma 5 to upper bound each term in the recursion, and together with an analysis on the influence of truncation, we could show that the first-order term will cancel out in the recursion and only the second-order term will be left. Thus, we show that for any  $\mathbf{c}_i^t$ , we have  $\rho_t(\mathbf{c}_i^t) = O(\sum_{t'=T-t+1}^T \frac{1}{t'})$ , which implies that  $\rho_1(\mathbf{c}_i^*) = O(\log T)$ . The complete proof is relegated to the appendix. Then, from (32), we could establish the following regret bound of Algorithm 2.

**Theorem 4** *Suppose Assumption 3 hold, then we have the following regret bound:*

$$\text{Regret}(ATP_1) \leq \sum_{i=1}^n \sum_{j=1}^m r_{ii_j} [(j+1)M - j] (\log T + 1) + \sum_{i=1}^n r_{\max}^i \cdot K_i = O(nm^2 \log T) \quad (35)$$

It is interesting to note that the re-solving procedure for each sub-problem in Algorithm 2 has also been applied to designing near-optimal policy for network revenue management problem with a so-called "non-degeneracy" assumption in Jasin and Kumar (2012) and following-up work Jasin (2015). We will conclude this subsection by making a comparison between our approach and their approach in the following remark.

**Remark:** a similarity between our approach and the approach in Jasin and Kumar (2012) and Jasin (2015) is that the optimal solution for the LP upper bound could be expressed in closed-form via the remaining capacity of each resource. However, our regret analysis is fundamentally different from theirs. A key step in their analysis is that they showed under the "non-degeneracy" assumption, the closed-form expression could be obtained provided that  $\frac{c_j^t}{T-t+1}$  for all  $j$ , where  $c_j^t$  denotes the remaining capacity of resource  $j$  at time  $t$ , doesn't variate too much from  $\frac{c_j}{T}$  so that the bases for the LP upper bound doesn't change. Then they showed that this condition could be guaranteed for a sufficiently long time in their policy by constructing a martingale involving  $\frac{c_j^t}{T-t+1}$  and applying the Doob's inequality for martingale. As a result, their regret bound is obtained when the ratio  $\frac{c_j}{T}$  is fixed and it's not clear how to generalize their approach to the setting where  $c_j$  could grow sublinearly in  $T$ . In contrast, our closed-form expression is obtained for any  $c_j^t$  and our regret analysis is based on considering the curvature of the distribution function of the size instead of constructing a martingale, thus our approach works for the setting where  $c_j$  is fixed and  $T \rightarrow \infty$ . Also, we need to analyze the influence of the fact that the actual threshold is truncated by the remaining capacity, which is not needed in their analysis since  $c_j$  grows linearly in  $T$  thus  $c_j^t$  will always exceeds the size of the request.

#### 4.4. Asymptotic Optimality

In this subsection we will proceed to study how does  $\mathbb{E}[V^{\text{off}}(\mathbf{I})]$  scale over  $T$ . Our next theorem shows that  $\mathbb{E}[V^{\text{off}}(\mathbf{I})] = \Omega(T^{\frac{1}{1+\alpha}})$ , where  $\alpha$  is a positive constant depending on  $\lambda, \gamma_1, \gamma_2$  in Assumption 3. Thus, we immediately show the asymptotic optimality of our adaptive threshold policy as  $T \rightarrow +\infty$ .

**Theorem 5** *Suppose Assumption 3 holds, then we have*

$$\mathbb{E}[V^{\text{off}}(\mathbf{I})] = \Omega(T^{\frac{1}{1+\alpha}}) \quad (36)$$

where  $\alpha$  is a positive constant satisfying  $\frac{1}{\gamma_2} = \lambda^\alpha$ .

### 5. Regret Bound for Resource-independent Case

The main purpose of this section is to study whether the term  $n$  in our previous  $O(\log T)$  regret bound could be removed and whether we could directly deal with our online resource allocation problem without reducing the problem into  $n$  separate problems. We show that under a special case where both the reward and the size of each request are resource-independent, we can indeed derive a similar adaptive threshold policy to achieve a  $O(\log T)$  regret bound without any dependence on  $n$ . The main difference of our analysis from the previous analysis is that we directly show the threshold structure of the prophet upper bound without dividing it into  $n$  sub-LPs. As a result, we could consider our online resource allocation problem as a whole without any reduction. Although we only analyze the case where the reward distribution has a finite support to keep the notation in consistent with the previous section, our analysis could be directly applied to the case where the support of the reward distribution is infinite and our regret bound continue to hold. In this section, we will make the following assumption:

**Assumption 4** *For each  $t$ , both  $\tilde{\mathbf{r}}^t$  and  $\tilde{\mathbf{d}}^t$  are single-dimensional random variables and the value of  $\tilde{\mathbf{r}}^t$  is drawn independently from  $\{r_1, r_2, \dots, r_n\}$ .*

In consistence with the previous section, we will use  $p_i$  to denote the probability that  $\tilde{\mathbf{r}}^t = r_i$  and use  $F_i(\cdot)$  to denote the distribution of  $\tilde{\mathbf{d}}^t$  given that  $\tilde{\mathbf{r}}^t = r_i$ . In what follows, we will first show the threshold structure of our prophet upper bound and then derive our policy and show the corresponding regret bound.

**Theorem 6** *We have the following upper bound of the expected total reward collected by the prophet:*

$$\mathbb{E}[V^{\text{off}}(\mathbf{I})] \leq T \cdot \sum_{i=1}^n p_i \cdot r_i \cdot F_i(r_i \cdot \mu(\mathbf{c})) \quad (37)$$

where the threshold  $\mu(\mathbf{c})$  is obtained by solving the following equation:

$$\sum_{i=1}^n p_i \cdot \int_0^{r_i \cdot \mu(\mathbf{c})} w_i dF_i(w_i) = \frac{\sum_{j=1}^m c_j}{T} \quad (38)$$

If there is no  $\mu(\mathbf{c})$  satisfying the above equation, then we set  $\mu(\mathbf{c}) = +\infty$ .

When the request arrives and reveals itself as  $(r_i, d)$ , based on the threshold structure of the prophet upper bound (37), we will make the accept/reject decision by comparing size  $d$  to the threshold  $r_i \cdot \mu$ , where we will compute the threshold  $\mu$  adaptively by (38). If the request is accepted, since the reward is resource-independent, it is natural for our policy to assign the resource with the largest capacity to serve it. Our policy is formally presented in Algorithm 3. Following a similar

---

**Algorithm 3** Adaptive Threshold Policy (ATP<sub>2</sub>)

---

- 1: At time period  $t = 1, 2, \dots, T$
- 2: Denote the remaining capacity as  $\mathbf{c}^t$ , and compute the threshold  $\mu_t(\mathbf{c}^t)$  by solving the equation

$$\sum_{i=1}^n p_i \cdot \int_0^{r_i \cdot \mu_t(\mathbf{c}^t)} w_i dF_i(w_i) = \frac{\sum_{j=1}^m c_j^t}{T - t + 1} \quad (39)$$

If there is no threshold  $\mu_t(\mathbf{c}^t)$  making the equation holds, then  $\mu_t(\mathbf{c}^t) = +\infty$ .

- 3: Denote  $j_t$  as the resource with largest remaining capacity, i.e.,  $c_{j_t}^t = \max\{c_1^t, c_2^t, \dots, c_m^t\}$ .
  - 4: For each  $i$ , define the truncated threshold  $h_t^i(\mathbf{c}^t) = \min\{c_{j_t}^t, r_i \cdot \mu_t(\mathbf{c}^t)\}$ .
  - 5: After request  $t$  arrives and reveals itself as  $(r_i, d)$ , do the following:
    - (i) Assign resource  $j_t$  to serve request  $t$  if  $d \leq h_t^i(\mathbf{c}^t)$ .
    - (ii) Reject request  $t$  if  $d > h_t^i(\mathbf{c}^t)$ .
- 

way of proving Lemma 6, we could obtain the following regret bound of Algorithm 3.

**Theorem 7** Suppose Assumption 3 holds and  $\hat{K}$  is the constant defined as follows:

$$\hat{K} = \left\lceil \frac{\sum_{j=1}^m c_j}{\sum_{i=1}^n p_i \cdot \int_0^{r_i \cdot \frac{\bar{w}}{r_{\max}}} w_i dF_i(w_i)} \right\rceil \quad (40)$$

where  $r_{\max} = \max\{r_1, r_2, \dots, r_n\}$ . Then we have the following regret bound

$$\text{Regret}(\text{ATP}_2) \leq (\log T + 1) \cdot (2mM - m) \cdot r_{\max} + r_{\max} \cdot \hat{K} = O(m \log T) \quad (41)$$

It is also worth-noting that when there is only one resource, then the *typical class* conditions from Arlotto and Xie (2020) is enough to establish the above regret bound. The reason is that in the proof, when there is only one resource, we will only need to bound the term  $\frac{wF(w)}{\int_0^w u dF(u)}$  and this term is upper bounded by a constant  $M$  under the *typical class* conditions due to Lemma 4 in Arlotto and Xie (2020). Also, Theorem 5 continues to hold and given the  $O(\log T)$  regret bound, Algorithm 3 is also asymptotically optimal as  $T \rightarrow \infty$ .

## 6. Concluding Remarks

In this paper, we considered a general model of the online resource allocation problem and we considered both the competitive ratio and the regret bound. For the most general case where both the size and the reward of the request could depend on which resource assigned, we proposed a nonadaptive threshold policy based on the optimal solution obtained from the prophet upper bound. We showed that our policy enjoys a competitive ratio of 0.302. Moreover, we showed that there doesn't exist an online algorithm with a competitive ratio larger than 0.5.

Then, we focused on the setting where  $T$  is large and considered our problem under two conditions separately: the reward could only take  $n$  values and both the reward and the size are independent of which resource assigned. Under each condition, we proposed an adaptive threshold policy and proved a  $O(\log T)$  regret bound. Our approaches for both conditions are based on showing that the optimal solution to the corresponding prophet upper bound possesses a threshold structure and we could mimick the prophet by following an adaptive threshold policy. Specifically, for the first condition, our policy will first divide each resource into  $n$  parts and will only use one specific part of each resource to serve the requests with the corresponding reward. As a result, the regret bound will depend on  $n$ . We then explored if there exists a policy without dividing the resources and if the regret bound will not depend on the cardinality of the support set of the reward. We showed that under the second condition, we could propose another adaptive threshold policy which utilizes each resource as a whole and we showed that the corresponding regret bound will be independent of  $n$ . Our analysis could be directly applied to the case where the cardinality of the support set of the reward is infinitely large and our regret bound continue to hold. Also, we showed that the expected reward collected by the prophet is at least  $\Omega(T^{\frac{1}{1+\alpha}})$  where  $\alpha$  is a positive constant depending on the distribution functions, thus, together with the  $O(\log T)$  regret bound, we established the asymptotic optimality of our policies.

Further research could be conducted in the following way: it is also interesting to investigate whether the  $O(\log T)$  regret bound will continue to hold when the reward and the size could depend on the resource assigned and the reward distribution is not finite support. Our future efforts will be devoted to solving this problem.

## Acknowledgments

The authors would like to thank Will Ma from Columbia University for helpful discussions.

## References

- Agrawal, Shipra, Zizhuo Wang, Yinyu Ye. 2014. A dynamic near-optimal algorithm for online linear programming. *Operations Research* **62**(4) 876–890.

- Alaei, Saeed, MohammadTaghi Hajiaghayi, Vahid Liaghat. 2013. The online stochastic generalized assignment problem. *Approximation, Randomization, and Combinatorial Optimization. Algorithms and Techniques*. Springer, 11–25.
- Arlotto, Alessandro, Itai Gurvich. 2019. Uniformly bounded regret in the multisecretary problem. *Stochastic Systems* **9**(3) 231–260.
- Arlotto, Alessandro, Xinchang Xie. 2020. Logarithmic regret in the dynamic and stochastic knapsack problem with equal rewards. *Stochastic Systems* .
- Brubach, Brian, Karthik Abinav Sankararaman, Aravind Srinivasan, Pan Xu. 2016. New algorithms, better bounds, and a novel model for online stochastic matching. *24th Annual European Symposium on Algorithms (ESA 2016)*. Schloss Dagstuhl-Leibniz-Zentrum fuer Informatik.
- Bruss, F Thomas, James B Robertson. 1991. wald’s lemma’for sums of order statistics of iid random variables. *Advances in applied probability* **23**(3) 612–623.
- Bumpensanti, Pornpawee, He Wang. 2020. A re-solving heuristic with uniformly bounded loss for network revenue management. *Management Science* .
- Coffman, EG, L Flatto, RR Weber. 1987. Optimal selection of stochastic intervals under a sum constraint. *Advances in applied probability* **19**(2) 454–473.
- Dean, Brian C, Michel X Goemans, Jan Vondrák. 2008. Approximating the stochastic knapsack problem: The benefit of adaptivity. *Mathematics of Operations Research* **33**(4) 945–964.
- Devanur, Nikhil R, Thomas P Hayes. 2009. The adwords problem: online keyword matching with budgeted bidders under random permutations. *Proceedings of the 10th ACM conference on Electronic commerce*. ACM, 71–78.
- Devanur, Nikhil R, Balasubramanian Sivan, Yossi Azar. 2012. Asymptotically optimal algorithm for stochastic adwords. *Proceedings of the 13th ACM Conference on Electronic Commerce*. 388–404.
- Dütting, Paul, Michal Feldman, Thomas Kesselheim, Brendan Lucier. 2017. Prophet inequalities made easy: Stochastic optimization by pricing non-stochastic inputs. *2017 IEEE 58th Annual Symposium on Foundations of Computer Science (FOCS)*. IEEE, 540–551.
- Feldman, Jon, Aranyak Mehta, Vahab Mirrokni, Shan Muthukrishnan. 2009. Online stochastic matching: Beating  $1-1/e$ . *2009 50th Annual IEEE Symposium on Foundations of Computer Science*. IEEE, 117–126.
- Freund, Daniel, Siddhartha Banerjee. 2019. Uniform loss algorithms for online stochastic decision-making with applications to bin packing. *Available at SSRN 3479189* .
- Goel, Gagan, Aranyak Mehta. 2008. Online budgeted matching in random input models with applications to adwords. *Proceedings of the nineteenth annual ACM-SIAM symposium on Discrete algorithms*. 982–991.

- Golrezaei, Negin, Hamid Nazerzadeh, Paat Rusmevichientong. 2014. Real-time optimization of personalized assortments. *Management Science* **60**(6) 1532–1551.
- Goyal, Vineet, Garud Iyengar, Rajan Udwani. 2020. Online allocation of reusable resources: Achieving optimal competitive ratio. *arXiv preprint arXiv:2002.02430* .
- Hernández-Lerma, Onésimo, Jean B Lasserre. 1998. Approximation schemes for infinite linear programs. *SIAM Journal on Optimization* **8**(4) 973–988.
- Jasin, Stefanus. 2015. Performance of an lp-based control for revenue management with unknown demand parameters. *Operations Research* **63**(4) 909–915.
- Jasin, Stefanus, Sunil Kumar. 2012. A re-solving heuristic with bounded revenue loss for network revenue management with customer choice. *Mathematics of Operations Research* **37**(2) 313–345.
- Karp, Richard M, Umesh V Vazirani, Vijay V Vazirani. 1990. An optimal algorithm for on-line bipartite matching. *Proceedings of the twenty-second annual ACM symposium on Theory of computing*. 352–358.
- Kesselheim, Thomas, Andreas Tönnis, Klaus Radke, Berthold Vöcking. 2014. Primal beats dual on online packing lps in the random-order model. *Proceedings of the forty-sixth annual ACM symposium on Theory of computing*. ACM, 303–312.
- Li, Xiaocheng, Yinyu Ye. 2019. Online linear programming: Dual convergence, new algorithms, and regret bounds. *arXiv preprint arXiv:1909.05499* .
- Lueker, George S. 1998. Average-case analysis of off-line and on-line knapsack problems. *Journal of Algorithms* **29**(2) 277–305.
- Ma, Will, David Simchi-Levi. 2019. Algorithms for online matching, assortment, and pricing with tight weight-dependent competitive ratios. *arXiv preprint arXiv:1905.04770* .
- Ma, Will, David Simchi-Levi, Jinglong Zhao. 2018. Dynamic pricing under a static calendar. *arXiv preprint arXiv:1811.01077* .
- Ma, Will, David Simchi-Levi, Jinglong Zhao. 2019. A competitive analysis of online knapsack problems with unit density. *arXiv preprint arXiv:1907.08735* .
- Marchetti-Spaccamela, Alberto, Carlo Vercellis. 1995. Stochastic on-line knapsack problems. *Mathematical Programming* **68**(1-3) 73–104.
- Mehta, Aranyak. 2013. Online matching and ad allocation. *Foundations and Trends® in Theoretical Computer Science* **8**(4) 265–368.
- Mehta, Aranyak, Amin Saberi, Umesh Vazirani, Vijay Vazirani. 2005. Adwords and generalized on-line matching. *46th Annual IEEE Symposium on Foundations of Computer Science (FOCS'05)*. IEEE, 264–273.
- Mirroknii, Vahab S, Shayan Oveis Gharan, Morteza Zadimoghaddam. 2012. Simultaneous approximations for adversarial and stochastic online budgeted allocation. *Proceedings of the twenty-third annual ACM-SIAM symposium on Discrete Algorithms*. SIAM, 1690–1701.



- Molinaro, Marco, Ramamoorthi Ravi. 2013. The geometry of online packing linear programs. *Mathematics of Operations Research* **39**(1) 46–59.
- Papastavrou, Jason D, Srikanth Rajagopalan, Anton J Kleywegt. 1996. The dynamic and stochastic knapsack problem with deadlines. *Management Science* **42**(12) 1706–1718.
- Rusmevichientong, Paat, Mika Sumida, Huseyin Topaloglu. 2020. Dynamic assortment optimization for reusable products with random usage durations. *Management Science* .
- Stein, Clifford, Van-Anh Truong, Xinshang Wang. 2019. Advance service reservations with heterogeneous customers. *Management Science* .
- Vera, Alberto, Siddhartha Banerjee. 2019. The bayesian prophet: A low-regret framework for online decision making. *Abstracts of the 2019 SIGMETRICS/Performance Joint International Conference on Measurement and Modeling of Computer Systems*. ACM, 81–82.
- Vera, Alberto, Siddhartha Banerjee, Itai Gurvich. 2019. Online allocation and pricing: Constant regret via bellman inequalities. *arXiv preprint arXiv:1906.06361* .
- Zhou, Yunhong, Deeparnab Chakrabarty, Rajan Lukose. 2008. Budget constrained bidding in keyword auctions and online knapsack problems. *International Workshop on Internet and Network Economics*. Springer, 566–576.

## Appendix. Proofs of Lemmas, Propositions and Theorems

### A. Proof of Claim 1

For each  $t$ , we could define a random variable  $Y^t$  such that  $Y_j^t \leq Y^t$  and  $E[Y^t] = \frac{c_j - u_j}{T}$ , then we must have

$$\sum_{t=1}^T P\left(\sum_{\tau=1}^{t-1} Y_j^\tau \leq \frac{c_j}{2}\right) \geq \sum_{t=1}^T P\left(\sum_{\tau=1}^{t-1} Y^\tau \leq \frac{c_j}{2}\right)$$

Following Lemma 6.1 in Dean et al. (2008), define  $S_t = \sum_{\tau=1}^t Y^\tau$  and denote  $\sigma_t = E[S_t | A_t]$ , where  $A_t$  is the event that  $S_t \leq \frac{c_j}{2}$ . Denote  $\bar{A}_t$  as the complement event of  $A_t$ , then we have

$$\begin{aligned} \sigma_t + E[Y^{t+1}] &= E[S_t | A_t] + E[Y^{t+1}] = E[S_t + Y^{t+1} | A_t] \\ &= E[S_{t+1} | A_{t+1}] \cdot P(A_{t+1} | A_t) + E[S_t + Y^{t+1} | \bar{A}_{t+1} \cap A_t] \cdot P(\bar{A}_{t+1} | A_t) \\ &\geq \sigma_{t+1} \cdot \frac{P(A_{t+1})}{P(A_t)} + \frac{c_j}{2} \cdot \left(1 - \frac{P(A_{t+1})}{P(A_t)}\right) \end{aligned}$$

which implies that

$$\frac{P(A_{t+1})}{P(A_t)} \geq \frac{c_j/2 - \sigma_t - E[Y^{t+1}]}{c_j/2 - \sigma_{t+1}} \quad (42)$$

For  $t = 0$ , we set  $P(A_0) = 1$  and  $\sigma_0 = 0$ . Then we consider two cases:

(i). For all  $t = 0, 1, 2, \dots, T-1$ , we have  $c_j/2 - \sigma_t - E[Y^{t+1}] \geq 0$ , then the RHS of (42) is always nonnegative, and by multiplying (42) from  $\tau = 0$  upto  $t-1$  for any  $t < T$ , we get

$$P(A_t) \geq \frac{c_j/2}{c_j/2 - \sigma_t} \cdot \prod_{\tau=0}^{t-1} \frac{c_j/2 - \sigma_\tau - E[Y^{\tau+1}]}{c_j/2 - \sigma_\tau} = \frac{c_j/2}{c_j/2 - \sigma_t} \cdot \prod_{\tau=0}^{t-1} \left(1 - \frac{E[Y^{\tau+1}]}{c_j/2 - \sigma_\tau}\right) \quad (43)$$

Define  $v_t = \frac{E[Y^{t+1}]}{c_j/2 - \sigma_t}$ , we get

$$\sum_{t=0}^{T-1} P(A_t) \cdot \frac{E[Y^{t+1}]}{c_j/2} \geq \sum_{t=0}^{T-1} v_t \cdot \prod_{\tau=0}^{t-1} (1 - v_\tau) = 1 - \prod_{t=0}^{T-1} (1 - v_t) \quad (44)$$

Moreover, since  $v_t = \frac{E[Y^{t+1}]}{c_j/2 - \sigma_t} \geq \frac{E[Y^{t+1}]}{c_j/2} = \frac{2(c_j - u_j)}{c_j T}$ , we get

$$\sum_{t=0}^{T-1} P(A_t) \geq \frac{c_j/2}{E[Y^{t+1}]} \cdot \left(1 - \left(1 - \frac{2(c_j - u_j)}{c_j T}\right)^T\right) \geq \frac{T c_j}{2(c_j - u_j)} \cdot \left(1 - e^{-\frac{2(c_j - u_j)}{c_j}}\right)$$

(ii). For some  $t < T$ , we have  $c_j/2 < \sigma_t + E[Y^{t+1}]$  and consider the smallest such  $t$ . Then  $c_j/2 - \sigma_\tau - E[Y^{\tau+1}] \geq 0$  for all  $\tau < t$ , and we could apply (44) to variables  $Y^1, Y^2, \dots, Y^t$  and get

$$\sum_{\tau=0}^{t-1} P(A_\tau) \cdot \frac{E[Y^{\tau+1}]}{c_j/2} \geq 1 - \prod_{\tau=0}^{t-1} (1 - v_\tau) \quad (45)$$

In addition, from (43), we have

$$P(A_t) \cdot \frac{E[Y^{t+1}]}{c_j/2} \geq P(A_t) \cdot \frac{c_j/2 - \sigma_t}{c_j/2} \geq \prod_{\tau=0}^{t-1} (1 - v_\tau) \quad (46)$$

Thus, we must have

$$\sum_{t=0}^{T-1} P(A_t) \geq \sum_{\tau=0}^t P(A_\tau) \geq \frac{T c_j}{2(c_j - u_j)} \cdot \left(1 - \prod_{\tau=0}^{t-1} (1 - v_\tau) + \prod_{\tau=0}^{t-1} (1 - v_\tau)\right) = \frac{T c_j}{2(c_j - u_j)}$$

which completes our proof.

## B. Solving the minimization problem in (18)

Denote  $a = u_j/c_j$  and define a function

$$G(a) = \frac{g^1(u_j) + g^2(u_j)}{g^1(u_j) \cdot g^2(u_j)} = \frac{2a}{1 - e^{-2a}} + \frac{2(1-a)}{1 - e^{-2(1-a)}}$$

Compute the derivative:

$$G'(a) = \frac{(2 - 2e^{-2a} - 4ae^{-2a})(1 - e^{-2(1-a)})^2 - (2 - 2e^{-2(1-a)} - 4(1-a)e^{-2(1-a)})(1 - e^{-2a})^2}{(1 - e^{-2a})^2(1 - e^{-2(1-a)})^2}$$

Since  $G'(a)$  is a single-variable function over  $(0, 1)$  and is a continuous function, we could simply discretize the interval  $(0, 1)$  and numerically show that  $G'(a) < 0$  for  $a \in (0, 0.5)$  and  $G'(a) > 0$  for  $a \in (0.5, 1)$ . Also, note that we have

$$\lim_{a \rightarrow 0+} G(a) = \frac{3 - e^{-2}}{1 - e^{-2}} \quad \text{and} \quad \lim_{a \rightarrow 1-} G(a) = \frac{3 - e^{-2}}{1 - e^{-2}}$$

Thus, we have  $G(a) \leq \frac{3 - e^{-2}}{1 - e^{-2}}$  for every  $a \in (0, 1)$ , which completes the proof of (18).

### C. Proof of Lemma 1

We will prove the lemma by showing that both relationships " $\leq$ ", " $\geq$ " hold between  $\text{LP}^{\text{UB}}$  and the right hand side of (23). We first prove " $\leq$ ". Denote  $\{x_j^*(\mathbf{r}_i, \mathbf{b}_i \cdot u)\}$  as the optimal solution of (6) and define  $\hat{c}_{ij} = T \cdot p_i \cdot b_{ij} \cdot \mathbb{E}_i[u \cdot x_j^*(\mathbf{r}_i, \mathbf{b}_i \cdot u)]$ . Obviously, the capacity constraints of (6) imply that  $\{\hat{c}_{ij}\}$  forms a feasible solution of the RHS of (23). Then we focus on  $G_i(\hat{\mathbf{c}}_i, 1)$  and denote  $\hat{x}_{ij}(u) = x_j^*(\mathbf{r}_i, \mathbf{b}_i \cdot u)$ . It is obvious that  $\{\hat{x}_{ij}(u)\}$  forms a feasible solution of (22), thus we have that

$$G_i(\hat{\mathbf{c}}_i, 1) \geq T \cdot p_i \cdot \mathbb{E}_i\left[\sum_{j=1}^m r_{ij} \cdot \hat{x}_{ij}(u)\right] = T \cdot p_i \cdot \mathbb{E}_i\left[\sum_{j=1}^m r_{ij} \cdot x_j^*(\mathbf{r}_i, \mathbf{b}_i \cdot u)\right]$$

which implies that

$$\text{LP}^{\text{UB}} = \sum_{i=1}^n T \cdot p_i \cdot \mathbb{E}_i\left[\sum_{j=1}^m r_{ij} \cdot x_j^*(\mathbf{r}_i, \mathbf{b}_i \cdot u)\right] \leq \sum_{i=1}^n G_i(\hat{\mathbf{c}}_i, 1) \leq \text{the RHS of (23)}$$

Next, we prove " $\geq$ ". Denote  $\{c_{ij}^*\}$  as the optimal solution of the RHS of (23) and denote  $\{x_{ij}^*(u)\}$  as the optimal solution of (22) for  $G_i(\mathbf{c}_i^*, 1)$ . Then we define  $\hat{x}_j(\mathbf{r}_i, \mathbf{b}_i \cdot u) = x_{ij}^*(u)$  and we have that

$$0 \leq \hat{x}_j(\mathbf{r}_i, \mathbf{b}_i \cdot u) \leq 1 \quad \text{and} \quad \sum_{j=1}^m \hat{x}_j(\mathbf{r}_i, \mathbf{b}_i \cdot u) = \sum_{j=1}^m x_{ij}^*(u) \leq 1$$

Also, we have that

$$T \cdot \mathbb{E}[b_{ij} \cdot u \cdot \hat{x}_j(\mathbf{r}_i, \mathbf{b}_i \cdot u)] = \sum_{i=1}^n T \cdot p_i \cdot b_{ij} \cdot \mathbb{E}_i[u \cdot \hat{x}_j(\mathbf{r}_i, \mathbf{b}_i \cdot u)] = \sum_{i=1}^n T \cdot p_i \cdot b_{ij} \cdot \mathbb{E}_i[u \cdot x_{ij}^*(u)] = \sum_{i=1}^n c_{ij}^* \leq c_j$$

Thus,  $\{\hat{x}_j(\mathbf{r}_i, \mathbf{b}_i \cdot u)\}$  forms a feasible solution of (6) and we have

$$\text{LP}^{\text{UB}} \geq \sum_{i=1}^n T \cdot p_i \cdot \mathbb{E}_i\left[\sum_{j=1}^m r_{ij} \cdot \hat{x}_j(\mathbf{r}_i, \mathbf{b}_i \cdot u)\right] = \sum_{i=1}^n T \cdot p_i \cdot \mathbb{E}_i\left[\sum_{j=1}^m r_{ij} \cdot x_{ij}^*(u)\right] = \sum_{i=1}^n G_i(\mathbf{c}_i^*, 1) = \text{the RHS of (23)}$$

which completes our proof.

### D. Proof of Lemma 2

We first show that  $G_i(\tilde{\mathbf{c}}_i, t) \leq (T - t + 1) \cdot p_i \cdot \sum_{j=1}^m (r_{ij} - r_{ii_{j+1}}) \cdot F_i(\mu_t^{ii_j}(\tilde{\mathbf{c}}_i))$ . Suppose  $\{x_{ii_j}^*(u)\}$  is the optimal solution of (22) and we define that  $\hat{y}_{ii_j}(u) = \sum_{k=1}^j x_{ii_k}^*(u)$  for each  $j$ , then it follows that

$$0 \leq \hat{y}_{ii_j}(u) \leq 1 \quad \text{and} \quad (T - t + 1) \cdot p_i \cdot \mathbb{E}_i[u \cdot \hat{y}_{ii_j}(u)] \leq \sum_{k=1}^j \tilde{c}_{ii_k} / b_{ii_k}$$

Then we define  $\hat{z}_{ij} = \mathbb{E}_i[\hat{y}_{ii_j}(u)]$  for each  $j$ . It is obvious that  $0 \leq \hat{z}_{ij} \leq 1$  and we also have the following constraint regarding  $\hat{z}_{ij}$

$$(T - t + 1) \cdot p_i \cdot \int_0^{F_i^{-1}(\hat{z}_{ij})} u dF_i(u) \leq (T - t + 1) \cdot p_i \cdot \mathbb{E}_i[u \cdot \hat{y}_{ii_j}(u)] \leq \sum_{k=1}^j \tilde{c}_{ii_k} / b_{ii_k} \quad (47)$$

The first inequality holds by noting that  $\hat{y}_{ii_j}(u) \in [0, 1]$ , then the expectation  $\mathbb{E}_i[u \cdot \hat{y}_{ii_j}(u)]$  must be lower bounded by integrating  $u$  from the smallest realization 0 to a realization  $a$  such that  $P(\{u \in [0, a]\}) = \mathbb{E}_i[\hat{y}_{ii_j}(u)] = \hat{z}_{i_j}$ . Also note that

$$\begin{aligned} G_i(\tilde{\mathbf{c}}_i, t) &= (T-t+1) \cdot p_i \cdot \sum_{j=1}^m r_{ii_j} \cdot \mathbb{E}_i[x_{ii_j}^*(u)] = (T-t+1) \cdot p_i \cdot \sum_{j=1}^m (r_{ii_j} - r_{ii_{j+1}}) \cdot \mathbb{E}_i[\hat{y}_{ii_j}(u)] \\ &= (T-t+1) \cdot p_i \cdot \sum_{j=1}^m (r_{ii_j} - r_{ii_{j+1}}) \cdot \hat{z}_{i_j} \end{aligned}$$

Thus, we have

$$\begin{aligned} G_i(\tilde{\mathbf{c}}_i, t) &\leq \max \quad (T-t+1) \cdot p_i \cdot \sum_{j=1}^m (r_{ii_j} - r_{ii_{j+1}}) \cdot z_{i_j} \\ \text{s.t.} \quad &(T-t+1) \cdot p_i \cdot \int_0^{F_i^{-1}(z_{i_j})} w dF_i(w) \leq \sum_{k=1}^j \tilde{c}_{ii_k} / b_{ii_k} \quad \forall j \\ &0 \leq z_{i_j} \leq 1 \quad \forall j \end{aligned} \tag{48}$$

Note that each constraint in the RHS of (48) only involves a single  $z_{i_j}$  and the objective function is linear in  $z_{i_j}$ , thus, the optimization problem is separable over  $\{z_{i_j}\}$  and for each  $j$ , the optimal solution  $z_{i_j}^*$  is given by solving the following single-variable optimization problem:

$$\begin{aligned} \max \quad &(T-t+1) \cdot p_i \cdot (r_{ii_j} - r_{ii_{j+1}}) \cdot z_{i_j} \\ \text{s.t.} \quad &(T-t+1) \cdot p_i \cdot \int_0^{F_i^{-1}(z_{i_j})} w dF_i(w) \leq \sum_{k=1}^j \tilde{c}_{ii_k} / b_{ii_k} \\ &0 \leq z_{i_j} \leq 1 \end{aligned}$$

Since  $r_{ii_j} - r_{ii_{j+1}} \geq 0$ , obviously the optimal solution  $z_{i_j}^*$  satisfies

$$(T-t+1) \cdot p_i \cdot \int_0^{F_i^{-1}(z_{i_j}^*)} w dF_i(w) = \sum_{k=1}^j \tilde{c}_{ii_k} / b_{ii_k}, \quad \text{if } (T-t+1) \cdot p_i \cdot \int_0^\infty w dF_i(w) \geq \sum_{k=1}^j \tilde{c}_{ii_k} / b_{ii_k}$$

and

$$z_{i_j}^* = 1, \quad \text{if } (T-t+1) \cdot p_i \cdot \int_0^\infty w dF_i(w) < \sum_{k=1}^j \tilde{c}_{ii_k} / b_{ii_k}$$

Thus, we have  $\mu_t^{ii_j}(\tilde{\mathbf{c}}_i) = F_i^{-1}(z_{i_j}^*)$  and it follows that  $G_i(\tilde{\mathbf{c}}_i, t) \leq (T-t+1) \cdot p_i \cdot \sum_{j=1}^m (r_{ii_j} - r_{ii_{j+1}}) \cdot F_i(\mu_t^{ii_j}(\tilde{\mathbf{c}}_i))$ . Note that

$$(T-t+1) \cdot p_i \cdot \mathbb{E}_i\left[\sum_{j=1}^m r_{ii_j} \cdot \hat{x}_{ii_j}(u)\right] = (T-t+1) \cdot p_i \cdot \sum_{j=1}^m (r_{ii_j} - r_{ii_{j+1}}) \cdot F_i(\mu_t^{ii_j}(\tilde{\mathbf{c}}_i))$$

It remains to show that  $\{\hat{x}_{ii_j}(u)\}$  is feasible to (22). Obviously for each  $u$ , we have that  $\sum_{j=1}^m \hat{x}_{ii_j}(u) \leq 1$  and for each  $j$ , we have that

$$(T-t+1) \cdot p_i \cdot \mathbb{E}_i[u \cdot \hat{x}_{ii_j}(u)] = (T-t+1) \cdot p_i \cdot \int_{\mu_t^{ii_{j-1}}(\tilde{\mathbf{c}}_i)}^{\mu_t^{ii_j}(\tilde{\mathbf{c}}_i)} u dF_i(u) \leq \tilde{c}_{ii_j} / b_{ii_j}$$

which completes our proof.

### E. Proof of Lemma 3

We will firstly show that under the condition, there exists two constants  $M_1, M_2 > 0$  such that

$$M_1 \leq \frac{wF(w)}{\int_0^w u dF(u)} \leq M_2 \quad \text{for all } w \in (0, \bar{w}) \quad (49)$$

The second inequality has already been established in Lemma 4 in Arlotto and Xie (2020) and the proof is replicated as follows for completeness:

$$\begin{aligned} 0 < 1 - \gamma_1 &\leq 1 - \frac{F(\lambda w)}{F(w)} = \int_{\lambda w}^w \frac{dF(u)}{F(w)} \quad \text{for all } w \in (0, \bar{w}) \\ \Rightarrow \lambda w(1 - \gamma_1) &\leq \int_{\lambda w}^w \frac{\lambda w}{F(w)} dF(u) \leq \int_0^w \frac{u}{F(w)} dF(u) \\ \Rightarrow \frac{wF(w)}{\int_0^w u dF(u)} &\leq \frac{1}{\lambda(1 - \gamma_1)} = M_2 \quad \text{for all } w \in (0, \bar{w}) \end{aligned}$$

Thus, we only focus on proving the first inequality. We have that for any  $w \in (0, \bar{w})$  and any positive integer  $k$ ,

$$1 - \frac{F(\lambda^k w)}{F(\lambda^{k-1} w)} \leq 1 - \frac{1}{\gamma_2} \Rightarrow \int_{\lambda^k w}^{\lambda^{k-1} w} \frac{dF(u)}{F(\lambda^{k-1} w)} \leq 1 - \frac{1}{\gamma_2}$$

then we have

$$\int_{\lambda^k w}^{\lambda^{k-1} w} \frac{u dF(u)}{F(\lambda^{k-1} w)} \leq \int_{\lambda^k w}^{\lambda^{k-1} w} \frac{\lambda^{k-1} w dF(u)}{F(\lambda^{k-1} w)} \leq (1 - \frac{1}{\gamma_2}) \cdot \lambda^{k-1} w$$

also, notice that  $\frac{1}{F(\lambda^{k-1} w)} \geq \gamma_1^{k-1} \cdot \frac{1}{F(w)}$ , we have

$$\int_{\lambda^k w}^{\lambda^{k-1} w} \frac{u dF(u)}{F(w)} \leq (1 - \frac{1}{\gamma_2}) \cdot (\frac{\lambda}{\gamma_1})^{k-1} w$$

Thus, it holds that

$$\int_0^w \frac{u dF(u)}{F(w)} = \sum_{k=1}^{+\infty} \int_{\lambda^k w}^{\lambda^{k-1} w} \frac{u dF(u)}{F(w)} \leq \sum_{k=1}^{+\infty} (1 - \frac{1}{\gamma_2}) \cdot (\frac{\lambda}{\gamma_1})^{k-1} w = \frac{w\gamma_1(\gamma_2 - 1)}{\gamma_1\gamma_2 - \lambda\gamma_2}$$

which implies

$$\frac{wF(w)}{\int_0^w u dF(u)} \geq \frac{\gamma_1\gamma_2 - \lambda\gamma_2}{\gamma_1(\gamma_2 - 1)}$$

and completes our proof of (49). Moreover, We could also find a positive integer  $l$  such that  $\frac{M_1}{\lambda^{l-1}} \leq M_2 \leq \frac{M_1}{\lambda^l}$ , then for any  $0 < w_1 < w_2 < \bar{w}$ , we consider two situations:

(i). If  $\lambda^l \cdot w_2 \leq w_1 < w_2$ , we have

$$\frac{w_2(F(w_2) - F(w_1))}{\int_{w_1}^{w_2} u dF(u)} \leq \frac{w_2(F(w_2) - F(w_1))}{\int_{w_1}^{w_2} w_1 dF(u)} = \frac{w_2}{w_1} \leq 1/\lambda^l$$

(ii). If  $w_1 < \lambda^l \cdot w_2$ , we have

$$w_2 \cdot F(w_1) \geq \frac{1}{\lambda^l} \cdot w_1 \cdot F(w_1) \geq \frac{M_1}{\lambda^l} \cdot \int_0^{w_1} u dF(u)$$

Thus, we have that

$$\begin{aligned} w_2(F(w_2) - F(w_1)) &\leq M_2 \cdot \int_0^{w_2} u dF(u) - \frac{M_1}{\lambda^l} \cdot \int_0^{w_1} u dF(u) = M_2 \cdot \int_{w_1}^{w_2} u dF(u) + (M_2 - \frac{M_1}{\lambda^l}) \cdot \int_0^{w_1} u dF(u) \\ &\leq M_2 \cdot \int_{w_1}^{w_2} u dF(u) \end{aligned}$$

Our proof is completed by setting  $M = \max\{\frac{1}{\lambda^l}, M_2\}$ .

## F. Proof of Lemma 4

Since  $F_i(\cdot)$  has a continuous density function  $f_i(\cdot)$ , implicit function theorem implies that the threshold  $\mu_t^{ii_j}(\tilde{\mathbf{c}}_i)$  is differentiable over  $\tilde{c}_{ii_k}$  and the derivatives can be obtained by taking derivative over both sides of (24). We have that

$$\frac{\partial \mu_t^{ii_j}(\tilde{\mathbf{c}}_i)}{\partial \tilde{c}_{ii_k}} = \frac{1}{p_i \cdot b_{ii_k} \cdot (T - t + 1) \cdot \mu_t^{ii_j}(\tilde{\mathbf{c}}_i) \cdot f_i(\mu_t^{ii_j}(\tilde{\mathbf{c}}_i))} \quad (50)$$

Thus, we have that

$$\frac{\partial}{\partial \tilde{c}_{ii_k}} \left( \frac{1}{\mu_t^{ii_j}(\tilde{\mathbf{c}}_i)} \right) = - \frac{1}{(\mu_t^{ii_j}(\tilde{\mathbf{c}}_i))^2} \cdot \frac{\partial \mu_t^{ii_j}(\tilde{\mathbf{c}}_i)}{\partial \tilde{c}_{ii_k}} = - \frac{1}{p_i \cdot b_{ii_k} \cdot (T - t + 1) \cdot (\mu_t^{ii_j}(\tilde{\mathbf{c}}_i))^3 \cdot f_i(\mu_t^{ii_j}(\tilde{\mathbf{c}}_i))}$$

From Condition 2 in Assumption 3,  $(\mu_t^{ii_j}(\tilde{\mathbf{c}}_i))^3 \cdot f_i(\mu_t^{ii_j}(\tilde{\mathbf{c}}_i))$  is a non-decreasing function over  $\mu_t^{ii_j}(\tilde{\mathbf{c}}_i)$ . Also, noting that  $\mu_t^{ii_j}(\tilde{\mathbf{c}}_i)$  is non-decreasing over  $\tilde{c}_{ii_k}$ , we have  $(\mu_t^{ii_j}(\tilde{\mathbf{c}}_i))^3 \cdot f_i(\mu_t^{ii_j}(\tilde{\mathbf{c}}_i))$  is a non-decreasing function over  $\tilde{c}_{ii_k}$ . Thus, we have that  $\frac{\partial}{\partial \tilde{c}_{ii_k}} \left( \frac{1}{\mu_t^{ii_j}(\tilde{\mathbf{c}}_i)} \right)$  is a non-decreasing function over  $\tilde{c}_{ii_k}$ , which implies the function  $\frac{1}{\mu_t^{ii_j}(\tilde{\mathbf{c}}_i)}$  is a convex function over  $\tilde{c}_{ii_k}$ .

## G. Proof of Lemma 5

First, note that

$$\frac{\partial F_i(\mu_t^{ii_j}(\tilde{\mathbf{c}}_i))}{\partial \tilde{c}_{ii_k}} = f_i(\mu_t^{ii_j}(\tilde{\mathbf{c}}_i)) \cdot \frac{\partial \mu_t^{ii_j}(\tilde{\mathbf{c}}_i)}{\partial \tilde{c}_{ii_k}} = \frac{1}{p_i \cdot b_{ii_k} \cdot (T - t + 1) \cdot \mu_t^{ii_j}(\tilde{\mathbf{c}}_i)} \quad (51)$$

which implies

$$p_i \cdot (T - t + 1) \cdot (F_i(\mu_t^{ii_j}(\tilde{\mathbf{c}}_i)) - F_i(\mu_t^{ii_j}(\tilde{\mathbf{c}}_i - b_{ii_k} \cdot u \cdot \mathbf{e}_{i_k}))) = \int_{\tilde{c}_{ii_k}/b_{ii_k} - u}^{\tilde{c}_{ii_k}/b_{ii_k}} \frac{1}{\mu_t^{ii_j}(\tilde{\mathbf{c}}_i - (\tilde{c}_{ii_k} - b_{ii_k} \cdot v) \cdot \mathbf{e}_{i_k})} dv \quad (52)$$

From Lemma 4, the function  $\frac{1}{\mu_t^{ii_j}(\tilde{\mathbf{c}}_i - (\tilde{c}_{ii_k} - b_{ii_k} \cdot v) \cdot \mathbf{e}_{i_k})}$  is a convex function over  $v$ , which implies that

$$\int_{\tilde{c}_{ii_k}/b_{ii_k} - u}^{\tilde{c}_{ii_k}/b_{ii_k}} \frac{1}{\mu_t^{ii_j}(\tilde{\mathbf{c}}_i - (\tilde{c}_{ii_k} - b_{ii_k} \cdot v) \cdot \mathbf{e}_{i_k})} dv \leq \frac{u}{2} \cdot \left[ \frac{1}{\mu_t^{ii_j}(\tilde{\mathbf{c}}_i)} + \frac{1}{\mu_t^{ii_j}(\tilde{\mathbf{c}}_i - b_{ii_k} \cdot u \cdot \mathbf{e}_{i_k})} \right] \quad (53)$$

Thus, we have that

$$p_i \cdot (T - t + 1) \cdot (F_i(\mu_t^{ii_j}(\tilde{\mathbf{c}}_i)) - F_i(\mu_t^{ii_j}(\tilde{\mathbf{c}}_i - u \cdot \mathbf{e}_{i_k}))) \leq \frac{u}{2} \cdot \left[ \frac{1}{\mu_t^{ii_j}(\tilde{\mathbf{c}}_i)} + \frac{1}{\mu_t^{ii_j}(\tilde{\mathbf{c}}_i - b_{ii_k} \cdot u \cdot \mathbf{e}_{i_k})} \right] \quad (54)$$

We then define a function  $g(u)$  as follows:

$$g(u) := \frac{p_i \cdot (T - t + 1)}{u^2} \cdot (F_i(\mu_t^{ii_j}(\tilde{\mathbf{c}})) - F_i(\mu_t^{ii_j}(\tilde{\mathbf{c}} - b_{ii_k} \cdot u \cdot \mathbf{e}_{i_k}))) - \frac{1}{u \cdot \mu_t^{ii_j}(\tilde{\mathbf{c}}_i)} \quad (55)$$

Then the derivative of  $g(u)$  over  $u$  could be obtained as follows:

$$\begin{aligned} g'(u) &= -\frac{2p_i(T-t+1)}{u^3} \cdot (F_i(\mu_t^{ii_j}(\tilde{\mathbf{c}}_i)) - F_i(\mu_t^{ii_j}(\tilde{\mathbf{c}}_i - b_{ii_k} u \cdot \mathbf{e}_{i_k}))) + \frac{1}{u^2} \cdot \left[ \frac{1}{\mu_t^{ii_j}(\tilde{\mathbf{c}}_i)} + \frac{1}{\mu_t^{ii_j}(\tilde{\mathbf{c}}_i - b_{ii_k} u \cdot \mathbf{e}_{i_k})} \right] \\ &= -\frac{2}{u^3} \left\{ p_i(T-t+1)(F_i(\mu_t^{ii_j}(\tilde{\mathbf{c}}_i)) - F_i(\mu_t^{ii_j}(\tilde{\mathbf{c}}_i - b_{ii_k} u \cdot \mathbf{e}_{i_k}))) - \frac{u}{2} \cdot \left[ \frac{1}{\mu_t^{ii_j}(\tilde{\mathbf{c}}_i)} + \frac{1}{\mu_t^{ii_j}(\tilde{\mathbf{c}}_i - b_{ii_k} u \cdot \mathbf{e}_{i_k})} \right] \right\} \end{aligned} \quad (56)$$

Thus, we have that  $g'(u) \geq 0$ , which implies that  $g(u) \leq g(\tilde{c}_{ii_k}/b_{ii_k})$ . Then we have

$$\begin{aligned} g(u) &= \frac{p_i(T-t+1)}{u^2} \cdot (F_i(\mu_t^{ii_j}(\tilde{\mathbf{c}}_i)) - F_i(\mu_t^{ii_j}(\tilde{\mathbf{c}}_i - b_{ii_k} u \cdot \mathbf{e}_{i_k}))) - \frac{1}{u \cdot \mu_t^{ii_j}(\tilde{\mathbf{c}}_i)} \\ &\leq g(\tilde{c}_{ii_k}/b_{ii_k}) = \frac{p_i(T-t+1)}{(\tilde{c}_{ii_k}/b_{ii_k})^2} \cdot (F_i(\mu_t^{ii_j}(\tilde{\mathbf{c}}_i)) - F_i(\mu_t^{ii_j}(\tilde{\mathbf{c}}_i - \tilde{c}_{ii_k} \cdot \mathbf{e}_{i_k}))) - \frac{1}{\tilde{c}_{ii_k}/b_{ii_k} \cdot \mu_t^{ii_j}(\tilde{\mathbf{c}}_i)} \end{aligned}$$

Thus, we have that

$$\begin{aligned} F_i(\mu_t^{ii_j}(\tilde{\mathbf{c}}_i)) - F_i(\mu_t^{ii_j}(\tilde{\mathbf{c}}_i - b_{ii_k} u \cdot \mathbf{e}_{i_k})) &\leq \frac{u^2}{(\tilde{c}_{ii_k}/b_{ii_k})^2} \cdot (F_i(\mu_t^{ii_j}(\tilde{\mathbf{c}}_i)) - F_i(\mu_t^{ii_j}(\tilde{\mathbf{c}}_i - \tilde{c}_{ii_k} \cdot \mathbf{e}_{i_k}))) \\ &\quad + \frac{u}{p_i \cdot (T-t+1) \cdot \mu_t^{ii_j}(\tilde{\mathbf{c}}_i)} - \frac{u^2}{\tilde{c}_{ii_k}/b_{ii_k} \cdot p_i(T-t+1) \cdot \mu_t^{ii_j}(\tilde{\mathbf{c}}_i)} \end{aligned}$$

Moreover, due to Lemma 3, we have that

$$\begin{aligned} \frac{\mu_t^{ii_j}(\tilde{\mathbf{c}}_i) \cdot (F_i(\mu_t^{ii_j}(\tilde{\mathbf{c}}_i)) - F_i(\mu_t^{ii_j}(\tilde{\mathbf{c}}_i - \tilde{c}_{ii_k} \cdot \mathbf{e}_{i_k})))}{\tilde{c}_{ii_k}} &= \frac{\mu_t^{ii_j}(\tilde{\mathbf{c}}_i) \cdot (F_i(\mu_t^{ii_j}(\tilde{\mathbf{c}}_i)) - F_i(\mu_t^{ii_j}(\tilde{\mathbf{c}}_i - \tilde{c}_{ii_k} \cdot \mathbf{e}_{i_k})))}{p_i b_{ii_k} (T-t+1) \cdot \int_{\mu_t^{ii_j}(\tilde{\mathbf{c}}_i - \tilde{c}_{ii_k} \cdot \mathbf{e}_{i_k})}^{\mu_t^{ii_j}(\tilde{\mathbf{c}}_i)} w dF_i(w)} \\ &\leq \frac{M}{p_i b_{ii_k} (T-t+1)} \end{aligned}$$

Thus, we have that

$$F_i(\mu_t^{ii_j}(\tilde{\mathbf{c}}_i)) - F_i(\mu_t^{ii_j}(\tilde{\mathbf{c}}_i - b_{ii_k} u \cdot \mathbf{e}_{i_k})) \leq \frac{(M-1) \cdot u^2}{\tilde{c}_{ii_k}/b_{ii_k} \cdot p_i \cdot (T-t+1) \cdot \mu_t^{ii_j}(\tilde{\mathbf{c}}_i)} + \frac{u}{p_i \cdot (T-t+1) \cdot \mu_t^{ii_j}(\tilde{\mathbf{c}}_i)}$$

which completes our proof.

## H. Proof of Lemma 6

Since we focus on a fixed  $i$  during the proof, we will omit the index  $i$  by using index  $j$  to denote index  $i_j$ , using  $\mu_t^j(\mathbf{c}^t)$  to denote  $\mu_t^{ii_j}(\mathbf{c}_i^t)$  and using  $b_j$  to denote  $b_{ii_j}$ .

We only focus on the time period  $t$  such that  $t < T - K$ . The reason is that for any  $t < T - K$ , we must have for each  $j$  and every possible remaining capacity  $\mathbf{c}^t$ , the threshold  $\mu_t^j(\mathbf{c}^t)$  will satisfy  $\mu_t^j(\mathbf{c}^t) < \bar{\omega}$ . Thus, by only focusing on  $t < T - K$ , the value of  $\mu_t^j(\mathbf{c}^t)$  is always finite and we could

fully exploit the two conditions over the distribution function proposed in Assumption 3. Since  $K$  is a constant independent of  $T$ , the cost of ignoring the last  $K$  time periods is at most a constant regret, which must be upper bounded by  $r_{\max} \cdot K$ . In what follows, we assume  $t < T - K$ . Define

$$\rho_t(\mathbf{c}^t) = (T - t + 1) \cdot p \cdot \sum_{j=1}^m (r_j - r_{j+1}) \cdot F(\mu_t^j(\mathbf{c}^t)) - V_t(\mathbf{c}^t) \quad (57)$$

where  $V_t(\mathbf{c}^t)$  is the "to-go" expected total reward collected by the policy, i.e., the expected cumulative reward collected by the policy from serving requests with reward  $\mathbf{r}_i$  from time period  $t$  to the last time period  $T$  given the remaining capacity at time period  $t$  is  $\mathbf{c}^t$ . Then our final goal is to bound  $\rho_1(\mathbf{c}^*)$ . Given the remaining capacity  $\mathbf{c}^t$  and the current time period  $t$ , denote  $\{j_1, j_2, \dots, j_W\}$  as a subset of  $\{1, 2, \dots, m\}$  where  $j_1 = 1$  and  $\{j_1, j_2, \dots, j_W\}$  satisfies that

$$h_t^1(\mathbf{c}^t) = h_t^{j_1}(\mathbf{c}^t) \leq h_t^{j_2}(\mathbf{c}^t) \leq \dots \leq h_t^{j_W}(\mathbf{c}^t) = \max\{h_t^1(\mathbf{c}^t), h_t^2(\mathbf{c}^t), \dots, h_t^m(\mathbf{c}^t)\}$$

and for each  $1 \leq w \leq W$  and every  $j$  such that  $j_w < j \leq j_{w+1} - 1$ , we must have  $h_t^j(\mathbf{c}^t) < h_t^{j_w}(\mathbf{c}^t)$ , where we set  $j_{W+1} = m + 1$ . Note that the definition of  $\{j_1, j_2, \dots, j_W\}$  will enable us to obtain the following relationship.

**Claim 2** For any  $1 \leq w \leq W$ , we must have

$$\mu_t^{j_w}(\mathbf{c}^t) \geq c_j^t / b_j \quad \text{for every } j \text{ such that } j_w < j \leq j_{w+1} - 1 \quad (58)$$

*Proof:* we have that  $\mu_t^{j_w}(\mathbf{c}^t) \geq h_t^{j_w}(\mathbf{c}^t) > h_t^j(\mathbf{c}^t)$  for any  $j$  such that  $j_w < j \leq j_{w+1} - 1$ . Also, it is obvious that  $\mu_t^{j_w}(\mathbf{c}^t) \leq \mu_t^j(\mathbf{c}^t)$  since  $j_w < j$ . Note that  $h_t^j(\mathbf{c}^t) = \min\{c_j^t / b_j, \mu_t^j(\mathbf{c}^t)\}$ , it must hold that  $\mu_t^{j_w}(\mathbf{c}^t) \geq c_j^t / b_j$ .  $\square$

Moreover, according to our policy in Algorithm 2, for each  $1 \leq w \leq W$ , request  $t$  with size  $\mathbf{b} \cdot u$  will be served by resource  $j_w$  if and only if  $h_t^{j_w-1}(\mathbf{c}^t) < u \leq h_t^{j_w}(\mathbf{c}^t)$ , where we set  $j_0 = 0$  and  $h_t^{j_0}(\mathbf{c}^t) = 0$ , and request  $t$  will be discarded if and only if  $u > h_t^{j_W}(\mathbf{c}^t)$ . Then, we can write down recursion of  $V_t(\mathbf{c}^t)$  as follows:

$$\begin{aligned} V_t(\mathbf{c}^t) &= (1 - p)V_{t+1}(\mathbf{c}^t) + p \cdot \sum_{w=1}^W \int_{h_t^{j_w-1}(\mathbf{c}^t)}^{h_t^{j_w}(\mathbf{c}^t)} \{r_{j_w} + V_{t+1}(\mathbf{c}^t - b_{j_w} u \cdot \mathbf{e}_{j_w})\} dF(u) + p \cdot (1 - F(h_t^{j_W}(\mathbf{c}^t))) \cdot V_{t+1}(\mathbf{c}^t) \\ &= (1 - p \cdot F(h_t^{j_W}(\mathbf{c}^t))) \cdot V_{t+1}(\mathbf{c}^t) + p \cdot \sum_{w=1}^W \int_{h_t^{j_w-1}(\mathbf{c}^t)}^{h_t^{j_w}(\mathbf{c}^t)} \{r_{j_w} + V_{t+1}(\mathbf{c}^t - b_{j_w} u \cdot \mathbf{e}_{j_w})\} dF(u) \end{aligned} \quad (59)$$

where  $\mathbf{e}_{j_w}$  denotes a  $m$  dimensional vector with 1 at  $j_w$ th component and 0 at other components. We could substitute  $V_t(\cdot)$  by  $(T - t + 1)p \cdot \sum_{j=1}^m (r_j - r_{j+1}) \cdot F(\mu_t^j(\cdot)) - \rho_t(\cdot)$  and substitute  $V_{t+1}(\cdot)$  by



$(T-t)p \cdot \sum_{j=1}^m (r_j - r_{j+1}) \cdot F(\mu_{t+1}^j(\cdot)) - \rho_{t+1}(\cdot)$  in the above recursion. Then we will get the recursion of  $\rho_t(\mathbf{c}^t)$  as follows:

$$\begin{aligned} (T-t+1)p \sum_{j=1}^m (r_j - r_{j+1}) F(\mu_t^j(\mathbf{c}^t)) - \rho_t(\mathbf{c}^t) &= (1 - pF(h_t^{jW}(\mathbf{c}^t))) \{ (T-t)p \sum_{j=1}^m (r_j - r_{j+1}) F(\mu_{t+1}^j(\mathbf{c}^t)) - \rho_{t+1}(\mathbf{c}^t) \} \\ &+ p \sum_{w=1}^W \int_{h_t^{jw-1}(\mathbf{c}^t)}^{h_t^{jw}(\mathbf{c}^t)} \{ r_{jw} + (T-t)p \sum_{k=1}^m (r_k - r_{k+1}) F(\mu_{t+1}^k(\mathbf{c}^t - b_{jw}u \cdot \mathbf{e}_{jw})) - \rho_{t+1}(\mathbf{c}^t - b_{jw}u \cdot \mathbf{e}_{jw}) \} dF(u) \end{aligned} \quad (60)$$

which implies that

$$\begin{aligned} \rho_t(\mathbf{c}^t) &= (1 - pF(h_t^{jW}(\mathbf{c}^t))) \cdot \rho_{t+1}(\mathbf{c}^t) + p \sum_{w=1}^W \int_{h_t^{jw-1}(\mathbf{c}^t)}^{h_t^{jw}(\mathbf{c}^t)} \rho_{t+1}(\mathbf{c}^t - b_{jw}u \cdot \mathbf{e}_{jw}) dF(u) \\ &+ \underbrace{p \cdot \sum_{j=1}^m (r_j - r_{j+1}) F(\mu_t^j(\mathbf{c}^t)) - p \cdot \sum_{w=1}^W r_{jw} \cdot (F(h_t^{jw}(\mathbf{c}^t)) - F(h_t^{jw-1}(\mathbf{c}^t)))}_{\text{I}} \\ &+ \underbrace{(T-t)p \cdot \sum_{j=1}^m (r_j - r_{j+1}) \cdot (F(\mu_t^j(\mathbf{c}^t)) - F(\mu_{t+1}^j(\mathbf{c}^t)))}_{\text{II}} \\ &+ \underbrace{p \cdot \sum_{w=1}^W \int_{h_t^{jw-1}(\mathbf{c}^t)}^{h_t^{jw}(\mathbf{c}^t)} \{ (T-t)p \sum_{k=1}^m (r_k - r_{k+1}) \cdot (F(\mu_{t+1}^k(\mathbf{c}^t)) - F(\mu_{t+1}^k(\mathbf{c}^t - b_{jw}u \cdot \mathbf{e}_{jw}))) \} dF(u)}_{\text{III}} \end{aligned} \quad (61)$$

Denote  $\bar{\rho}_{t+1}$  as the maximal value of  $\rho_{t+1}(\mathbf{c}^{t+1})$  for all the possible remaining capacity  $\mathbf{c}^{t+1}$ . Then we have

$$\rho_t(\mathbf{c}^t) - \bar{\rho}_{t+1} \leq \text{I} + \text{II} + \text{III}$$

In the following, we will bound the three terms I, II, III separately.

**Bound I:** By rearranging terms, we get

$$\begin{aligned} \text{I} &= p \cdot \sum_{j=1}^m (r_j - r_{j+1}) F(\mu_t^j(\mathbf{c}^t)) - p \cdot \sum_{w=1}^W r_{jw} \cdot (F(h_t^{jw}(\mathbf{c}^t)) - F(h_t^{jw-1}(\mathbf{c}^t))) \\ &= p \cdot \sum_{w=1}^W \left\{ \sum_{j=j_w}^{j_{w+1}-1} (r_j - r_{j+1}) \cdot [F(\mu_t^j(\mathbf{c}^t)) - F(h_t^{jw}(\mathbf{c}^t))] \right\} \end{aligned} \quad (62)$$

Then, for each fixed  $j$  such that  $j_w \leq j \leq j_{w+1} - 1$ , we will bound the term  $F(\mu_t^j(\mathbf{c}^t)) - F(h_t^{jw}(\mathbf{c}^t))$ .

We will first prove the following bound.

**Claim 3** For each  $1 \leq w \leq W$  and each  $j$  such that  $j_w \leq j \leq j_{w+1} - 1$ , we must have

$$F(\mu_t^j(\mathbf{c}^t)) - F(h_t^{jw}(\mathbf{c}^t)) \leq \frac{M \cdot (j - j_w)}{p \cdot (T - t + 1)} + [F(\mu_t^{j_w}(\mathbf{c}^t)) - F(h_t^{j_w}(\mathbf{c}^t))] \cdot 1_{\{c_{j_w}^t / b_{j_w} < \mu_t^{j_w}(\mathbf{c}^t)\}} \quad (63)$$

*Proof:* note that from Lemma 3, we have that

$$\mu_t^j(\mathbf{c}^t) \cdot (F(\mu_t^j(\mathbf{c}^t)) - F(\mu_t^{jw}(\mathbf{c}^t))) \leq M \cdot \int_{\mu_t^{jw}(\mathbf{c}^t)}^{\mu_t^j(\mathbf{c}^t)} u dF(u) = \frac{M \cdot (c_{jw+1}^t/b_{jw+1} + \dots + c_j^t/b_j)}{p \cdot (T-t+1)} \quad (64)$$

Thus, we have

$$\begin{aligned} F(\mu_t^j(\mathbf{c}^t)) - F(h_t^{jw}(\mathbf{c}^t)) &= F(\mu_t^j(\mathbf{c}^t)) - F(\mu_t^{jw}(\mathbf{c}^t)) + F(\mu_t^{jw}(\mathbf{c}^t)) - F(h_t^{jw}(\mathbf{c}^t)) \\ &\leq \frac{M \cdot (c_{jw+1}^t/b_{jw+1} + \dots + c_j^t/b_j)}{\mu_t^j(\mathbf{c}^t) \cdot p \cdot (T-t+1)} + F(\mu_t^{jw}(\mathbf{c}^t)) - F(h_t^{jw}(\mathbf{c}^t)) \\ &\leq \frac{M \cdot (j - j_w)}{p \cdot (T-t+1)} + F(\mu_t^{jw}(\mathbf{c}^t)) - F(h_t^{jw}(\mathbf{c}^t)) \end{aligned} \quad (65)$$

where the first inequality holds due to (64) and the second inequality holds by noting that according to (58), we must have

$$\mu_t^j(\mathbf{c}^t) \geq \mu_t^{jw}(\mathbf{c}^t) \geq \max\{c_{jw+1}^t/b_{jw+1}, \dots, c_j^t/b_j\}$$

Note that  $h_t^{jw}(\mathbf{c}^t) = \min\{c_{jw}^t/b_{jw}, \mu_t^{jw}(\mathbf{c}^t)\}$ , then  $h_t^{jw}(\mathbf{c}^t)$  differentiates from  $\mu_t^{jw}(\mathbf{c}^t)$  if and only if  $c_{jw}^t/b_{jw} < \mu_t^{jw}(\mathbf{c}^t)$ , thus we have

$$F(\mu_t^j(\mathbf{c}^t)) - F(h_t^{jw}(\mathbf{c}^t)) \leq \frac{M \cdot (j - j_w)}{p \cdot (T-t+1)} + [F(\mu_t^{jw}(\mathbf{c}^t)) - F(h_t^{jw}(\mathbf{c}^t))] \cdot 1_{\{c_{jw}^t/b_{jw} < \mu_t^{jw}(\mathbf{c}^t)\}}$$

□

We then bound the term  $[F(\mu_t^{jw}(\mathbf{c}^t)) - F(h_t^{jw}(\mathbf{c}^t))] \cdot 1_{\{c_{jw}^t/b_{jw} < \mu_t^{jw}(\mathbf{c}^t)\}}$ .

**Claim 4** For any  $1 \leq w \leq W$ , it holds that

$$[F(\mu_t^{jw}(\mathbf{c}^t)) - F(h_t^{jw}(\mathbf{c}^t))] \cdot 1_{\{c_{jw}^t/b_{jw} < \mu_t^{jw}(\mathbf{c}^t)\}} \leq \frac{M \cdot j_w}{p \cdot (T-t+1)} \quad (66)$$

*Proof:* we will prove (66) by induction. For  $j_1 = 1$ , we have that

$$\begin{aligned} [F(\mu_t^{j_1}(\mathbf{c}^t)) - F(h_t^{j_1}(\mathbf{c}^t))] \cdot 1_{\{c_{j_1}^t/b_{j_1} < \mu_t^{j_1}(\mathbf{c}^t)\}} &\leq F(\mu_t^{j_1}(\mathbf{c}^t)) \cdot 1_{\{c_{j_1}^t/b_{j_1} < \mu_t^{j_1}(\mathbf{c}^t)\}} \\ &\leq \frac{M \cdot c_{j_1}^t/b_{j_1}}{\mu_t^{j_1}(\mathbf{c}^t) \cdot p \cdot (T-t+1)} \cdot 1_{\{c_{j_1}^t/b_{j_1} < \mu_t^{j_1}(\mathbf{c}^t)\}} \\ &\leq \frac{M}{p \cdot (T-t+1)} \end{aligned}$$

where the second inequality holds due to Lemma 3. Now suppose that

$$[F(\mu_t^{j_{w-1}}(\mathbf{c}^t)) - F(h_t^{j_{w-1}}(\mathbf{c}^t))] \cdot 1_{\{c_{j_{w-1}}^t/b_{j_{w-1}} < \mu_t^{j_{w-1}}(\mathbf{c}^t)\}} \leq \frac{M \cdot j_{w-1}}{p \cdot (T-t+1)}$$

then noting that  $h_t^{jw-1}(\mathbf{c}^t) \leq h_t^{jw}(\mathbf{c}^t)$ , we have

$$\begin{aligned}
& [F(\mu_t^{jw}(\mathbf{c}^t)) - F(h_t^{jw}(\mathbf{c}^t))] \cdot 1_{\{c_{jw}^t/b_{jw} < \mu_t^{jw}(\mathbf{c}^t)\}} \\
& \leq [F(\mu_t^{jw}(\mathbf{c}^t)) - F(\mu_t^{jw-1}(\mathbf{c}^t)) + F(\mu_t^{jw-1}(\mathbf{c}^t)) - F(h_t^{jw-1}(\mathbf{c}^t))] \cdot 1_{\{c_{jw}^t/b_{jw} < \mu_t^{jw}(\mathbf{c}^t)\}} \\
& \leq [F(\mu_t^{jw}(\mathbf{c}^t)) - F(\mu_t^{jw-1}(\mathbf{c}^t))] \cdot 1_{\{c_{jw}^t/b_{jw} < \mu_t^{jw}(\mathbf{c}^t)\}} + F(\mu_t^{jw-1}(\mathbf{c}^t)) - F(h_t^{jw-1}(\mathbf{c}^t)) \\
& = [F(\mu_t^{jw}(\mathbf{c}^t)) - F(\mu_t^{jw-1}(\mathbf{c}^t))] \cdot 1_{\{c_{jw}^t/b_{jw} < \mu_t^{jw}(\mathbf{c}^t)\}} + [F(\mu_t^{jw-1}(\mathbf{c}^t)) - F(h_t^{jw-1}(\mathbf{c}^t))] \cdot 1_{\{c_{jw-1}^t/b_{jw-1} < \mu_t^{jw-1}(\mathbf{c}^t)\}} \\
& \leq [F(\mu_t^{jw}(\mathbf{c}^t)) - F(\mu_t^{jw-1}(\mathbf{c}^t))] \cdot 1_{\{c_{jw}^t/b_{jw} < \mu_t^{jw}(\mathbf{c}^t)\}} + \frac{M \cdot j_{w-1}}{p \cdot (T - t + 1)}
\end{aligned}$$

Note that from Lemma 3, we have that

$$\begin{aligned}
& [F(\mu_t^{jw}(\mathbf{c}^t)) - F(\mu_t^{jw-1}(\mathbf{c}^t))] \cdot 1_{\{c_{jw}^t/b_{jw} < \mu_t^{jw}(\mathbf{c}^t)\}} \leq \frac{M \cdot (c_{jw-1+1}^t/b_{jw-1+1} + \dots + c_{jw}^t/b_{jw})}{\mu_t^{jw}(\mathbf{c}^t) \cdot p \cdot (T - t + 1)} \cdot 1_{\{c_{jw}^t/b_{jw} < \mu_t^{jw}(\mathbf{c}^t)\}} \\
& \leq \frac{M \cdot (c_{jw-1+1}^t/b_{jw-1+1} + \dots + c_{jw-1}^t/b_{jw-1})}{\mu_t^{jw}(\mathbf{c}^t) \cdot p \cdot (T - t + 1)} + \frac{M \cdot c_{jw}^t/b_{jw}}{\mu_t^{jw}(\mathbf{c}^t) \cdot p \cdot (T - t + 1)} \cdot 1_{\{c_{jw}^t/b_{jw} < \mu_t^{jw}(\mathbf{c}^t)\}} \\
& \leq \frac{M \cdot (c_{jw-1+1}^t/b_{jw-1+1} + \dots + c_{jw-1}^t/b_{jw-1})}{\mu_t^{jw}(\mathbf{c}^t) \cdot p \cdot (T - t + 1)} + \frac{M}{p \cdot (T - t + 1)} \\
& \leq \frac{M \cdot (j_w - 1 - j_{w-1})}{p \cdot (T - t + 1)} + \frac{M}{p \cdot (T - t + 1)} = \frac{M \cdot (j_w - j_{w-1})}{p \cdot (T - t + 1)}
\end{aligned}$$

where the last inequality holds by noting that according to (58), we must have

$$\mu_t^{jw}(\mathbf{c}^t) \geq \mu_t^{jw-1}(\mathbf{c}^t) \geq \max\{c_{jw-1+1}^t/b_{jw-1+1}, \dots, c_{jw-1}^t/b_{jw-1}\}$$

Thus, by induction, for any  $1 \leq w \leq W$ , (66) holds.  $\square$

Thus from (63) and (66), we have that

$$F(\mu_t^j(\mathbf{c}^t)) - F(h_t^{jw}(\mathbf{c}^t)) \leq \frac{M \cdot j}{p \cdot (T - t + 1)} \quad (67)$$

Then by substituting (67) into (62), we can finally upper bound the term I by:

$$I \leq \frac{M}{T - t + 1} \cdot \sum_{j=1}^m (r_j - r_{j+1}) \cdot j = \frac{M}{T - t + 1} \cdot \sum_{j=1}^m r_j \quad (68)$$

We then proceed to bound the term II.

**Bound II:** From the definition of the threshold  $\mu_t^j(\mathbf{c}^t)$  in (24), for each  $j = 1, 2, \dots, m$ , we have that

$$\frac{c_1^t/b_1 + \dots + c_j^t/b_j}{T - t} - \frac{c_1^t/b_1 + \dots + c_j^t/b_j}{T - t + 1} = p \cdot \int_{\mu_t^j(\mathbf{c}^t)}^{\mu_{t+1}^j(\mathbf{c}^t)} u dF(u) \leq p \cdot \mu_{t+1}^j(\mathbf{c}^t) \cdot [F(\mu_{t+1}^j(\mathbf{c}^t)) - F(\mu_t^j(\mathbf{c}^t))]$$

which implies

$$(T - t) \cdot p \cdot [F(\mu_t^j(\mathbf{c}^t)) - F(\mu_{t+1}^j(\mathbf{c}^t))] \leq - \frac{c_1^t/b_1 + \dots + c_j^t/b_j}{\mu_{t+1}^j(\mathbf{c}^t) \cdot (T - t + 1)}$$

Thus, we have the following upper bound regarding the term II:

$$\text{II} \leq - \sum_{j=1}^m (r_j - r_{j+1}) \cdot \frac{c_1^t/b_1 + \dots + c_j^t/b_j}{\mu_{t+1}^j(\mathbf{c}^t) \cdot (T - t + 1)} \quad (69)$$

At last, it remains to bound the term III.

**Bound III:** We begin with an observation that from the definition of the threshold  $\mu_t^j(\mathbf{c}^t)$  in (24), if  $k < j_w$ , then for any  $u$ , we must have  $\mu_{t+1}^k(\mathbf{c}^t) = \mu_{t+1}^k(\mathbf{c}^t - b_{j_w} u \cdot \mathbf{e}_{j_w})$ . Thus, we could rewrite the term III as:

$$\text{III} = p \cdot \sum_{w=1}^W \int_{h_t^{j_w-1}(\mathbf{c}^t)}^{h_t^{j_w}(\mathbf{c}^t)} \left\{ (T-t) \cdot p \cdot \sum_{k=j_w}^m (r_k - r_{k+1}) \cdot (F(\mu_{t+1}^k(\mathbf{c}^t)) - F(\mu_{t+1}^k(\mathbf{c}^t - b_{j_w} u \cdot \mathbf{e}_{j_w}))) \right\} dF(u) \quad (70)$$

Note that from Lemma 5, for any  $k \geq j_w$ , we have that

$$p(T-t) \cdot (F(\mu_{t+1}^k(\mathbf{c}^t)) - F(\mu_{t+1}^k(\mathbf{c}^t - b_{j_w} u \cdot \mathbf{e}_{j_w}))) \leq \frac{(M-1)u^2}{(c_{j_w}^t/b_{j_w}) \cdot \mu_{t+1}^k(\mathbf{c}^t)} + \frac{u}{\mu_{t+1}^k(\mathbf{c}^t)}$$

Then, we have that

$$\begin{aligned} \text{III} &\leq p(M-1) \cdot \underbrace{\sum_{w=1}^W \int_{h_t^{j_w-1}(\mathbf{c}^t)}^{h_t^{j_w}(\mathbf{c}^t)} \left\{ \sum_{k=j_w}^m (r_k - r_{k+1}) \cdot \frac{u^2}{(c_{j_w}^t/b_{j_w}) \cdot \mu_{t+1}^k(\mathbf{c}^t)} \right\} dF(u)}_{\text{IV}} \\ &\quad + p \cdot \underbrace{\sum_{w=1}^W \int_{h_t^{j_w-1}(\mathbf{c}^t)}^{h_t^{j_w}(\mathbf{c}^t)} \sum_{k=j_w}^m (r_k - r_{k+1}) \cdot \frac{u}{\mu_{t+1}^k(\mathbf{c}^t)} dF(u)}_{\text{V}} \end{aligned} \quad (71)$$

We next bound the term IV and V separately. We have that

$$\begin{aligned} \text{IV} &= p(M-1) \sum_{w=1}^W \sum_{k=j_w}^m \frac{r_k - r_{k+1}}{(c_{j_w}^t/b_{j_w}) \cdot \mu_{t+1}^k(\mathbf{c}^t)} \cdot \int_{h_t^{j_w-1}(\mathbf{c}^t)}^{h_t^{j_w}(\mathbf{c}^t)} u^2 dF(u) \\ &\leq p(M-1) \sum_{w=1}^W \sum_{k=j_w}^m \frac{r_k - r_{k+1}}{(c_{j_w}^t/b_{j_w}) \cdot \mu_{t+1}^k(\mathbf{c}^t)} \cdot h_t^{j_w}(\mathbf{c}^t) \cdot \int_{h_t^{j_w-1}(\mathbf{c}^t)}^{h_t^{j_w}(\mathbf{c}^t)} u dF(u) \\ &\leq p(M-1) \sum_{w=1}^W \sum_{k=j_w}^m \frac{r_k - r_{k+1}}{(c_{j_w}^t/b_{j_w})} \cdot \int_{h_t^{j_w-1}(\mathbf{c}^t)}^{h_t^{j_w}(\mathbf{c}^t)} u dF(u) \end{aligned} \quad (72)$$

where the second inequality holds by noting that when  $k \geq j_w$ , we must have  $h_t^{j_w}(\mathbf{c}^t) \leq \mu_t^{j_w}(\mathbf{c}^t) \leq \mu_t^k(\mathbf{c}^t) \leq \mu_{t+1}^k(\mathbf{c}^t)$ . We then bound the term  $\frac{1}{c_{j_w}^t/b_{j_w}} \cdot \int_{h_t^{j_w-1}(\mathbf{c}^t)}^{h_t^{j_w}(\mathbf{c}^t)} u dF(u)$  in (72).

**Claim 5** For any  $1 \leq w \leq W$ , it holds that

$$\frac{1}{c_{j_w}^t/b_{j_w}} \cdot \int_{h_t^{j_w-1}(\mathbf{c}^t)}^{h_t^{j_w}(\mathbf{c}^t)} u dF(u) \leq \frac{j_w}{p(T-t+1)} \quad (73)$$

*Proof:* For each  $j_w$ , we define the index  $j(w)$ :

$$j(w) := \max\{j : 0 \leq j < j_w \text{ and } c_j/b_j \geq \mu_t^j(\mathbf{c}^t)\} \quad (74)$$

where we will denote  $c_0 = \mu_t^0(\mathbf{c}^t) = 0$  and such a  $j(w)$  always exist. Since  $j(w) < j_w$ , from the definition of  $\{j_1, j_2, \dots, j_W\}$ , it must hold that

$$\mu_t^{j(w)}(\mathbf{c}^t) = h_t^{j(w)}(\mathbf{c}^t) \leq h_t^{j_w-1}(\mathbf{c}^t)$$

then we have

$$\begin{aligned} \frac{1}{c_{j_w}^t/b_{j_w}} \cdot \int_{h_t^{j_w-1}(\mathbf{c}^t)}^{h_t^{j(w)}(\mathbf{c}^t)} u dF(u) &\leq \frac{1}{c_{j_w}^t/b_{j_w}} \cdot \int_{h_t^{j(w)}(\mathbf{c}^t)}^{h_t^{j(w)}(\mathbf{c}^t)} u dF(u) \leq \frac{1}{c_{j_w}^t/b_{j_w}} \cdot \int_{\mu_t^{j(w)}(\mathbf{c}^t)}^{\mu_t^{j(w)}(\mathbf{c}^t)} u dF(u) \\ &= \frac{1}{c_{j_w}^t/b_{j_w}} \cdot \frac{c_{j(w)+1}^t/b_{j(w)+1} + \dots + c_{j_w}^t/b_{j_w}}{p(T-t+1)} \end{aligned}$$

where the last equality holds due to the definition of  $\mu_t^{j(w)}(\mathbf{c}^t)$  and  $\mu_t^{j_w}(\mathbf{c}^t)$  in (22). Moreover, note that from the definition of the index  $j(w)$ , for any index  $q$  such that  $j(w) < q < j_w$ , it must hold  $c_q^t/b_q < \mu_t^q(\mathbf{c}^t)$ . Thus, we have that  $c_q^t/b_q = h_t^q(\mathbf{c}^t) \leq h_t^{j(w)}(\mathbf{c}^t) \leq c_{j_w}^t/b_{j_w}$ , which implies that

$$\frac{c_{j(w)+1}^t/b_{j(w)+1} + \dots + c_{j_w}^t/b_{j_w}}{c_{j_w}^t/b_{j_w}} \leq j_w - j(w) \leq j_w$$

Thus, the proof is completed.  $\square$

By substituting (73) into (72), we conclude that

$$\text{IV} \leq \frac{M-1}{T-t+1} \cdot \sum_{w=1}^W \sum_{k=j_w}^m (r_k - r_{k+1}) j_w = \frac{M-1}{T-t+1} \cdot \sum_{w=1}^W r_{j_w} \cdot j_w \leq \frac{M-1}{T-t+1} \cdot \sum_{j=1}^m j \cdot r_j \quad (75)$$

At last, we bound the term V as follows:

$$\begin{aligned} \text{V} &= p \cdot \sum_{w=1}^W \int_{h_t^{j_w-1}(\mathbf{c}^t)}^{h_t^{j(w)}(\mathbf{c}^t)} \sum_{k=j_w}^m (r_k - r_{k+1}) \cdot \frac{u}{\mu_{t+1}^k(\mathbf{c}^t)} dF(u) = p \cdot \sum_{k=1}^m \frac{r_k - r_{k+1}}{\mu_{t+1}^k(\mathbf{c}^t)} \cdot \sum_{j_w: j_w \leq k} \int_{h_t^{j_w-1}(\mathbf{c}^t)}^{h_t^{j(w)}(\mathbf{c}^t)} u dF(u) \\ &\leq p \cdot \sum_{k=1}^m \frac{r_k - r_{k+1}}{\mu_{t+1}^k(\mathbf{c}^t)} \cdot \int_0^{\mu_t^k(\mathbf{c}^t)} u dF(u) = \sum_{k=1}^m (r_k - r_{k+1}) \cdot \frac{c_1^t/b_1 + \dots + c_k^t/b_k}{\mu_{t+1}^k(\mathbf{c}^t) \cdot (T-t+1)} \end{aligned} \quad (76)$$

where the first inequality holds by noting that for all  $j_w \leq k$ , we have  $h_t^{j(w)}(\mathbf{c}^t) \leq \mu_t^{j(w)}(\mathbf{c}^t) \leq \mu_t^k(\mathbf{c}^t)$ .

Finally, we can bound term III by:

$$\text{III} \leq \text{IV} + \text{V} \leq \frac{M-1}{T-t+1} \cdot \sum_{j=1}^m j \cdot r_j + \sum_{k=1}^m (r_k - r_{k+1}) \cdot \frac{c_1^t/b_1 + \dots + c_k^t/b_k}{\mu_{t+1}^k(\mathbf{c}^t) \cdot (T-t+1)} \quad (77)$$

By combining (68), (69) and (77), we have

$$\begin{aligned}
\rho_t(\mathbf{c}^t) - \bar{\rho}_{t+1} &\leq \frac{M}{T-t+1} \cdot \sum_{j=1}^m r_j - \sum_{j=1}^m (r_j - r_{j+1}) \cdot \frac{c_1^t/b_1 + \dots + c_j^t/b_j}{\mu_{t+1}^j(\mathbf{c}^t) \cdot (T-t+1)} \\
&\quad + \frac{M-1}{T-t+1} \cdot \sum_{j=1}^m j \cdot r_j + \sum_{k=1}^m (r_k - r_{k+1}) \cdot \frac{c_1^t/b_1 + \dots + c_k^t/b_k}{\mu_{t+1}^k(\mathbf{c}^t) \cdot (T-t+1)} \\
&= \frac{1}{T-t+1} \cdot \sum_{j=1}^m r_j \cdot (M(j+1) - j)
\end{aligned} \tag{78}$$

holds for any  $\mathbf{c}^t$ , which implies that

$$\bar{\rho}_t - \bar{\rho}_{t+1} \leq \frac{1}{T-t+1} \cdot \sum_{j=1}^m r_j \cdot (M(j+1) - j)$$

Thus, by noting that  $\bar{\rho}_{T-K+1} \leq r_{\max} \cdot K$ , we have

$$\begin{aligned}
\rho_1(\mathbf{c}^*) &\leq \bar{\rho}_1 \leq \sum_{t=1}^{T-K} (\bar{\rho}_t - \bar{\rho}_{t+1}) + \bar{\rho}_{T-K+1} \leq \sum_{t=1}^{T-K} \left( \frac{1}{T-t+1} \right) \cdot \sum_{j=1}^m (r_j \cdot (M(j+1) - j)) + r_{\max} \cdot K \\
&\leq (\log T + 1) \cdot \sum_{j=1}^m (r_j \cdot (M(j+1) - j)) + r_{\max} \cdot K
\end{aligned}$$

which completes our proof.

## I. Proof of Theorem 5

Since we have shown

$$\mathbb{E}[V^{\text{off}}(\mathbf{I})] \geq \mathbb{E}[V^{\text{ATP}_1}(\mathbf{I})] \geq \sum_{i=1}^n G_i(\mathbf{c}_i^*, 1) - O(\log T)$$

it is enough to show that  $\sum_{i=1}^n G_i(\mathbf{c}_i^*, 1) = \Omega(T^{\frac{1}{1+\alpha}})$ . Also, there must exists a  $i$  and  $i_j$  such that  $p_i > 0$ ,  $r_{ii_j} - r_{ii_{j+1}} > 0$  and  $\sum_{k=1}^j c_{ii_k}^* \geq \frac{\sum_{j=1}^m c_j}{n}$ . If we can show that

$$T \cdot p_i \cdot (r_{ii_j} - r_{ii_{j+1}}) \cdot F_i(\mu_1^{ii_j}(\mathbf{c}_i^*)) = \Omega(T^{\frac{1}{1+\alpha}})$$

then the proof is completed immediately. In what follows, we will use  $\mu_T$  to denote the threshold  $\mu_1^{ii_j}(\mathbf{c}_i^*)$  and denote  $l$  as the positive integer such that  $\lambda^l \cdot \bar{\omega} \leq \mu_T \leq \lambda^{l+1} \cdot \bar{\omega}$ . Then we have

$$\frac{\sum_{k=1}^j c_{ii_k}^*}{\bar{b} \cdot p_i \cdot T} \geq \frac{\sum_{k=1}^j c_{ii_k}^* / b_{ii_k}}{p_i \cdot T} = \int_0^{\mu_T} u dF_i(u) \geq \sum_{k=l}^{+\infty} \int_{\lambda^{k+1}\bar{\omega}}^{\lambda^k\bar{\omega}} u dF_i(u)$$

where  $\bar{b} = \min_{1 \leq k \leq j} \{b_{ii_k}\}$ . We also have that

$$\int_{\lambda^{k+1}\bar{\omega}}^{\lambda^k\bar{\omega}} u dF_i(u) \geq \lambda^{k+1}\bar{\omega} \cdot [F_i(\lambda^k\bar{\omega}) - F_i(\lambda^{k+1}\bar{\omega})] \geq \lambda^{k+1}\bar{\omega}(\gamma_1 - 1) \cdot F_i(\lambda^{k+1}\bar{\omega}) \geq \left(\frac{\lambda}{\gamma_2}\right)^{k+1}\bar{\omega}(\gamma_1 - 1)F_i(\bar{\omega})$$

The last inequality holds by noting  $F_i(\bar{\omega}) \leq \gamma_2^{k+1} \cdot F_i(\lambda^{k+1}\bar{\omega})$ . Thus, we have that

$$\frac{\sum_{k=1}^j c_{ii_k}^*}{\bar{b} \cdot p_i \cdot T} \geq \bar{\omega}(\gamma_1 - 1)F_i(\bar{\omega}) \cdot \sum_{k=l}^{+\infty} \left(\frac{\lambda}{\gamma_2}\right)^{k+1} = \bar{\omega}(\gamma_1 - 1)F_i(\bar{\omega}) \left(\frac{\lambda}{\gamma_2}\right)^{l+1} \cdot \frac{\gamma_2}{\gamma_2 - \lambda}$$

Define a constant  $Q = \frac{(\sum_{k=1}^j c_{ii_k}^*) \cdot (\gamma_2 - \lambda)}{\bar{b}\bar{\omega}(\gamma_1 - 1)\lambda p_i F_i(\bar{\omega})}$ , we have that

$$\left(\frac{\lambda}{\gamma_2}\right)^l \leq \frac{Q}{T}$$

Also, since  $0 < \lambda < 1$  and  $0 < \frac{1}{\gamma_2} < 1$ , there exists a constant  $\alpha > 0$  such that  $\frac{1}{\gamma_2} = \lambda^\alpha$ . Thus, we have

$$\lambda^{(1+\alpha)l} \leq \frac{Q}{T} \Rightarrow \lambda^l \leq \left(\frac{Q}{T}\right)^{\frac{1}{1+\alpha}}$$

Noting that from (49), we obtain that

$$F_i(\mu_T) \geq \frac{M_1}{\mu_T} \cdot \int_0^{\mu_T} u dF_i(u) = \frac{M_1 \cdot (\sum_{k=1}^j c_{ii_k}^* / b_{ii_k})}{\mu_T \cdot T} \geq \frac{M_1 \lambda (\sum_{k=1}^j c_{ii_k}^*)}{\hat{b} \cdot \bar{\omega} \cdot T} \cdot \frac{1}{\lambda^l}$$

where  $\hat{b} = \max_{1 \leq k \leq j} \{b_{ii_k}\}$ . Thus, we have that

$$\begin{aligned} T \cdot p_i \cdot (r_{ii_j} - r_{ii_{j+1}}) \cdot F_i(\mu_T) &\geq \frac{M_1 \lambda (r_{ii_j} - r_{ii_{j+1}}) (\sum_{k=1}^j c_{ii_k}^*)}{\hat{b} \cdot \bar{\omega}} \cdot \frac{1}{\lambda^l} \\ &\geq \frac{M_1 \lambda^{\frac{2+\alpha}{1+\alpha}} (r_{ii_j} - r_{ii_{j+1}}) ((\gamma_1 - 1) \bar{b} p_i F_i(\bar{\omega}))^{\frac{1}{1+\alpha}}}{\hat{b} \bar{\omega}^{\frac{\alpha}{1+\alpha}} (\gamma_2 - \lambda)^{\frac{1}{1+\alpha}}} \cdot \left(\sum_{k=1}^j c_{ii_k}^*\right)^{\frac{\alpha}{1+\alpha}} \cdot T^{\frac{1}{1+\alpha}} \\ &\geq \frac{M_1 \lambda^{\frac{2+\alpha}{1+\alpha}} (r_{ii_j} - r_{ii_{j+1}}) ((\gamma_1 - 1) \bar{b} p_i F_i(\bar{\omega}))^{\frac{1}{1+\alpha}} (\sum_{j=1}^m c_j)^{\frac{\alpha}{1+\alpha}}}{\hat{b} \bar{\omega}^{\frac{\alpha}{1+\alpha}} (\gamma_2 - \lambda)^{\frac{1}{1+\alpha}} n^{\frac{\alpha}{1+\alpha}}} \cdot T^{\frac{1}{1+\alpha}} \\ &= \Omega(T^{\frac{1}{1+\alpha}}) \end{aligned}$$

which completes our proof.

## J. Proof of Theorem 6

First, we have that

$$\begin{aligned} \text{LP}^{\text{UB}} &\leq \max \quad T \cdot \sum_{i=1}^n p_i \cdot \mathbb{E}_i[r_i \cdot y_i(d)] \\ \text{s.t.} \quad &T \cdot \sum_{i=1}^n p_i \cdot \mathbb{E}_i[d \cdot y_i(d)] \leq \sum_{j=1}^m c_j \\ &0 \leq y_i(d) \leq 1 \quad \forall d, \forall i \end{aligned} \tag{79}$$

The inequality holds by noting that the solution  $\{\hat{y}_i(d)\}$  defined by  $\hat{y}_i(d) = \sum_{j=1}^m x_j^*(r_i, d)$ , where  $\{x_j^*(r_i, d)\}$  is the optimal solution of (6), is feasible to the RHS of (79), and we have

$$\text{LP}^{\text{UB}} = T \cdot \sum_{i=1}^n p_i \cdot \mathbb{E}_i \left[ \sum_{j=1}^m r_i \cdot x_j^*(r_i, d) \right] = T \cdot \sum_{i=1}^n p_i \cdot \mathbb{E}_i [r_i \cdot \hat{y}_i(d)]$$

Suppose the optimal solution of the RHS of (79) is  $\{y_i^*(d)\}$ , then denote  $\hat{z}_i = \mathbb{E}_i[y_i^*(d)] \in [0, 1]$  for every  $i$  and similar to (47), we have the following constraint regarding  $\hat{z}_i$ :

$$\sum_{j=1}^m c_j \geq T \cdot \sum_{i=1}^n p_i \cdot \mathbb{E}_i[d \cdot y_i^*(d)] \geq T \cdot \sum_{i=1}^n p_i \cdot \left[ \int_0^{F_i^{-1}(\hat{z}_i)} w_i dF_i(w_i) \right] = T \cdot \sum_{i=1}^n p_i \cdot \left[ \int_0^{\hat{z}_i} F_i^{-1}(v_i) dv_i \right] \quad (80)$$

The last equality holds by replacing variable  $w_i$  by  $F_i^{-1}(v_i)$ . Thus, we have

$$\begin{aligned} \text{LP}^{\text{UB}} \leq \max \quad & T \cdot \sum_{i=1}^n p_i \cdot r_i \cdot z_i \\ \text{s.t.} \quad & T \cdot \sum_{i=1}^n p_i \cdot \int_0^{z_i} F_i^{-1}(v_i) dv_i \leq \sum_{j=1}^m c_j \\ & 0 \leq z_i \leq 1 \quad \forall i \end{aligned} \quad (81)$$

The RHS of (81) is a convex optimization problem over  $\{z_i\}$  by noting that for each  $i$ , if we define  $g_i(z) = \int_0^z F_i^{-1}(v) dv$ , then  $g'_i(z) = F_i^{-1}(z)$  is a non-decreasing function over  $z$ , which implies that  $g_i(z)$  is a convex function over  $z$ . Then strong duality implies that

$$\text{LP}^{\text{UB}} \leq \min_{\mu \geq 0} \max_{0 \leq z_i \leq 1} L(\mathbf{z}, \mu) \quad (82)$$

where  $L(\mathbf{z}, \mu)$  is the lagrangian function defined as follows:

$$L(\mathbf{z}, \mu) = T \cdot \sum_{i=1}^n r_i \cdot p_i \cdot z_i + \mu \cdot \left[ \sum_{j=1}^m c_j - T \cdot \sum_{i=1}^n p_i \cdot \int_0^{z_i} F_i^{-1}(v_i) dv_i \right] \quad (83)$$

Denote  $\{z_i^*, \mu^*\}$  as the optimal solution of the dual problem, then from the KKT condition, we have that

$$\frac{\partial L(\mathbf{z}^*, \mu^*)}{\partial z_i} = 0 \Rightarrow r_i \cdot p_i = \mu^* \cdot p_i \cdot F_i^{-1}(z_i^*) \Rightarrow z_i^* = F_i\left(\frac{r_i}{\mu^*}\right) \quad (84)$$

and

$$\mu^* \cdot \left[ \sum_{j=1}^m c_j - T \cdot \sum_{i=1}^n p_i \cdot \int_0^{z_i^*} F_i^{-1}(v_i) dv_i \right] = 0 \quad (85)$$

Then,  $\mu^* > 0$  will imply

$$\sum_{j=1}^m c_j - T \cdot \sum_{i=1}^n p_i \cdot \int_0^{z_i^*} F_i^{-1}(v_i) dv_i = 0 \Rightarrow \sum_{j=1}^m c_j - T \cdot \sum_{i=1}^n p_i \cdot \int_0^{F_i^{-1}(\frac{r_i}{\mu^*})} F_i^{-1}(v_i) dv_i = 0$$

Thus, we can have the following optimal solution  $z_i^* = F_i(\frac{r_i}{\mu^*})$  where  $\mu^*$  is obtained by solving the following equation:

$$T \cdot \sum_{i=1}^n p_i \cdot \int_0^{\frac{r_i}{\mu^*}} w_i dF_i(w_i) = T \cdot \sum_{i=1}^n p_i \cdot \int_0^{F_i^{-1}(\frac{r_i}{\mu^*})} F_i^{-1}(v_i) dv_i = \sum_{j=1}^m c_j$$

If no  $\mu^*$  makes the above equation hold, then  $\mu^* = 0$ . Thus, we have  $\mu(\mathbf{c}) = 1/\mu^*$ , which implies

$$\text{LP}^{\text{UB}} \leq \min_{\mu \geq 0} \max_{0 \leq z_i \leq 1} L(\mathbf{z}, \mu) = T \cdot \sum_{i=1}^n p_i \cdot r_i \cdot F_i(r_i \cdot \mu(\mathbf{c}))$$



## K. Proof of Theorem 7

We first prove the following lemma regarding the threshold  $\mu_t(\mathbf{c}^t)$ .

**Lemma 7** *For any  $j = 1, 2, \dots, m$ , the function  $\frac{1}{\mu_t(\mathbf{c}^t)}$  is a convex function over  $c_j^t$ .*

*Proof:* Since for each  $i$ ,  $F_i(\cdot)$  has a continuous density function  $f_i(\cdot)$ , then implicit function theorem tells us that the threshold  $\mu_t(\mathbf{c}^t)$  is differentiable over  $c_j^t$  for each  $j$  and the derivatives can be obtained by taking derivative over both sides of (39). We have that

$$\frac{\partial \mu_t(\mathbf{c}^t)}{\partial c_j^t} = \frac{1}{\sum_{i=1}^n p_i \cdot (T-t+1) \cdot r_i^2 \cdot \mu_t^j(\mathbf{c}^t) \cdot f_i(r_i \mu_t^j(\mathbf{c}^t))}$$

Thus, we have the function  $\frac{1}{\mu_t(\mathbf{c}^t)}$  is differentiable over  $c_j^t$  and we have that

$$\frac{\partial}{\partial c_j^t} \left( \frac{1}{\mu_t(\mathbf{c}^t)} \right) = -\frac{1}{(\mu_t(\mathbf{c}^t))^2} \cdot \frac{\partial \mu_t(\mathbf{c}^t)}{\partial c_j^t} = -\frac{1}{\sum_{i=1}^n \frac{p_i(T-t+1)}{r_i} \cdot (r_i \mu_t(\mathbf{c}^t))^3 \cdot f_i(r_i \mu_t(\mathbf{c}^t))}$$

From Condition 2 in Assumption 3, for each  $i$ , we have that  $(r_i \mu_t(\mathbf{c}^t))^3 \cdot f_i(r_i \mu_t(\mathbf{c}^t))$  is a non-decreasing function over  $r_i \mu_t(\mathbf{c}^t)$ . Also, obviously  $r_i \mu_t(\mathbf{c}^t)$  is non-decreasing over  $c_j^t$ , thus we get  $(r_i \mu_t(\mathbf{c}^t))^3 \cdot f_i(r_i \mu_t(\mathbf{c}^t))$  is a non-decreasing function over  $c_j^t$ . Finally, we have that  $\frac{\partial}{\partial c_j^t} \left( \frac{1}{\mu_t(\mathbf{c}^t)} \right)$  is a non-decreasing function over  $c_j^t$ , which implies the function  $\frac{1}{\mu_t(\mathbf{c}^t)}$  is a convex function over  $c_j^t$ .  $\square$

To derive the regret bound, we study the gap between the expected total reward collected by our policy and the prophet upper bound in Theorem 6. Specifically, define

$$\rho_t(\mathbf{c}^t) = (T-t+1) \cdot \sum_{i=1}^n p_i \cdot r_i \cdot F_i(r_i \mu_t(\mathbf{c}^t)) - V_t(\mathbf{c}^t) \quad (86)$$

where  $V_t(\mathbf{c}^t)$  is the "to-go" expected total reward collected by the our policy, i.e., the expected cumulative reward collected by our policy from time period  $t$  to the last time period  $T$  given the remaining capacity at time period  $t$  is denoted as  $\mathbf{c}^t$ . Then we have that

$$\text{Regret}(\text{ATP}_2) \leq \rho_1(\mathbf{c})$$

Since  $j_t$  is denoted as the resource with largest remaining capacity given the remaining capacity is  $\mathbf{c}^t$ , i.e.,  $c_{j_t}^t = \max\{c_1^t, c_2^t, \dots, c_m^t\}$ , and our policy will assign resource  $j_t$  to serve request  $t$ , revealed as  $(r_i, d)$ , as long as  $d \leq h_t^i(\mathbf{c}^t) = \min\{c_{j_t}^t, r_i \mu_t(\mathbf{c}^t)\}$ , we have the following recursion of  $V_t(\mathbf{c}^t)$ :

$$V_t(\mathbf{c}^t) = (1 - \sum_{i=1}^n p_i) V_{t+1}(\mathbf{c}^t) + \sum_{i=1}^n p_i \cdot \int_0^{h_t^i(\mathbf{c}^t)} \{r_i + V_{t+1}(\mathbf{c}^t - w_i \cdot \mathbf{e}_{j_t})\} dF_i(w_i) + \sum_{i=1}^n p_i (1 - F_i(h_t^i(\mathbf{c}^t))) V_{t+1}(\mathbf{c}^t)$$

$\Rightarrow$

$$V_t(\mathbf{c}^t) = (1 - \sum_{i=1}^n p_i F_i(h_t^i(\mathbf{c}^t))) V_{t+1}(\mathbf{c}^t) + \sum_{i=1}^n p_i \cdot \int_0^{h_t^i(\mathbf{c}^t)} \{r_i + V_{t+1}(\mathbf{c}^t - w_i \cdot \mathbf{e}_{j_t})\} dF_i(w_i)$$

where  $\mathbf{e}_{j_t}$  denotes a  $m$  dimensional vector with 1 at  $j_t$ th component and 0 at other components. Then, by substituting (86) into the above equation, we get the recursion of  $\rho_t(\mathbf{c}^t)$ .

$$(T-t+1) \cdot \sum_{i=1}^n p_i r_i F_i(r_i \mu_t(\mathbf{c}^t)) - \rho_t(\mathbf{c}^t) = (1 - \sum_{i=1}^n p_i F_i(h_t^i(\mathbf{c}^t))) \cdot [(T-t) \sum_{i=1}^n p_i r_i F_i(r_i \mu_{t+1}(\mathbf{c}^t)) - \rho_{t+1}(\mathbf{c}^t)] \\ + \sum_{i=1}^m p_i \cdot \int_0^{h_t^i(\mathbf{c}^t)} \{r_i + (T-t) \sum_{k=1}^n p_k r_k F_k(r_k \mu_{t+1}(\mathbf{c}^t - w_i \cdot \mathbf{e}_{j_t})) - \rho_{t+1}(\mathbf{c}^t - w_i \cdot \mathbf{e}_{j_t})\} dF_i(w_i)$$

which implies that

$$\begin{aligned} \rho_t(\mathbf{c}^t) &= (1 - \sum_{i=1}^n p_i F_i(h_t^i(\mathbf{c}^t))) \cdot \rho_{t+1}(\mathbf{c}^t) + \sum_{i=1}^n p_i \cdot \int_0^{h_t^i(\mathbf{c}^t)} \rho_{t+1}(\mathbf{c}^t - w_i \cdot \mathbf{e}_{j_t}) dF_i(w_i) \\ &+ \underbrace{\sum_{i=1}^n p_i r_i \cdot (F_i(r_i \mu_t(\mathbf{c}^t)) - F_i(h_t^i(\mathbf{c}^t)))}_{\text{I}} + \underbrace{(T-t) \cdot \sum_{i=1}^n p_i r_i \cdot (F_i(r_i \mu_t(\mathbf{c}^t)) - F_i(r_i \mu_{t+1}(\mathbf{c}^t)))}_{\text{II}} \\ &+ \underbrace{\sum_{i=1}^n p_i \cdot \int_0^{h_t^i(\mathbf{c}^t)} \{(T-t) \cdot \sum_{k=1}^n p_k r_k \cdot (F_k(r_k \mu_{t+1}(\mathbf{c}^t)) - F_k(r_k \mu_{t+1}(\mathbf{c}^t - w_i \cdot \mathbf{e}_{j_t})))\} dF_i(w_i)}_{\text{III}} \end{aligned}$$

By denoting  $\bar{\rho}_{t+1}$  as the maximal value of  $\rho_{t+1}(\mathbf{c}^{t+1})$  for all the possible remaining capacity  $\mathbf{c}^{t+1}$ .

Then we have

$$\rho_t(\mathbf{c}^t) - \bar{\rho}_{t+1} \leq \text{I} + \text{II} + \text{III}$$

In the following, we will bound the term I, II, III separately.

**Bound I:** From Lemma 3, we have that

$$\frac{r_i \mu_t(\mathbf{c}^t) F_i(r_i \mu_t(\mathbf{c}^t))}{\int_0^{r_i \mu_t(\mathbf{c}^t)} w_i dF_i(w_i)} \leq M \quad \forall i \Rightarrow \frac{\sum_{i=1}^n p_i r_i \mu_t(\mathbf{c}^t) F_i(r_i \mu_t(\mathbf{c}^t))}{\sum_{i=1}^n p_i \cdot \int_0^{r_i \mu_t(\mathbf{c}^t)} w_i dF_i(w_i)} \leq M$$

Also from the definition of  $\mu_t(\mathbf{c}^t)$  in (39), we have that

$$\sum_{i=1}^n p_i r_i \mu_t(\mathbf{c}^t) F_i(r_i \mu_t(\mathbf{c}^t)) \leq \frac{M \cdot (c_1^t + \dots + c_m^t)}{T-t+1}$$

Thus, note that  $h_t^i(\mathbf{c}^t) = \min\{c_{j_t}^t, r_i \cdot \mu_t(\mathbf{c}^t)\}$ , we have the following bound over the term I:

$$\begin{aligned} \text{I} &= \sum_{i=1}^n p_i r_i \cdot (F_i(r_i \mu_t(\mathbf{c}^t)) - F_i(h_t^i(\mathbf{c}^t))) \leq \sum_{i=1}^n p_i r_i F_i(r_i \mu_t(\mathbf{c}^t)) \cdot 1_{\{r_i \cdot \mu_t(\mathbf{c}^t) > c_{j_t}^t\}} \\ &\leq \sum_{i=1}^n p_i r_i F_i(r_i \mu_t(\mathbf{c}^t)) \cdot 1_{\{r_{\max} \cdot \mu_t(\mathbf{c}^t) > c_{j_t}^t\}} = 1_{\{r_{\max} \cdot \mu_t(\mathbf{c}^t) > c_{j_t}^t\}} \cdot \sum_{i=1}^n p_i r_i F_i(r_i \mu_t(\mathbf{c}^t)) \\ &\leq 1_{\{r_{\max} \cdot \mu_t(\mathbf{c}^t) > c_{j_t}^t\}} \cdot \frac{M \cdot (c_1^t + \dots + c_m^t)}{\mu_t(\mathbf{c}^t) \cdot (T-t+1)} \leq \frac{M \cdot (c_1^t + \dots + c_m^t) \cdot r_{\max}}{c_{j_t}^t \cdot (T-t+1)} \\ &\leq \frac{M \cdot r_{\max} \cdot m}{T-t+1} \end{aligned}$$

where  $r_{\max} = \{r_1, r_2, \dots, r_n\}$ . In the next, we bound the term II.

**Bound II:** From the definition of  $\mu_t(\mathbf{c}^t)$  in (39), we have

$$\frac{c_1^t + \dots + c_m^t}{T-t} - \frac{c_1^t + \dots + c_m^t}{T-t+1} = \sum_{i=1}^n p_i \cdot \int_{r_i \mu_t(\mathbf{c}^t)}^{r_i \mu_{t+1}(\mathbf{c}^t)} w_i dF_i(w_i) \leq \sum_{i=1}^n p_i r_i \mu_{t+1}(\mathbf{c}^t) \cdot (F_i(r_i \mu_{t+1}(\mathbf{c}^t)) - F_i(r_i \mu_t(\mathbf{c}^t)))$$

Thus, we have that

$$\text{II} = (T-t) \cdot \sum_{i=1}^n p_i r_i \cdot (F_i(r_i \mu_t(\mathbf{c}^t)) - F_i(r_i \mu_{t+1}(\mathbf{c}^t))) \leq -\frac{c_1^t + \dots + c_m^t}{\mu_{t+1}(\mathbf{c}^t) \cdot (T-t+1)}$$

At last, it remains to bound III.

**Bound III:** Note that

$$\frac{\partial \mu_{t+1}(\mathbf{c}^t)}{\partial c_{jt}^t} = \frac{1}{(T-t) \cdot \sum_{i=1}^n p_i r_i^2 f_i(r_i \mu_{t+1}(\mathbf{c}^t)) \cdot \mu_{t+1}(\mathbf{c}^t)}$$

Thus, we have that

$$\frac{\partial}{\partial c_{jt}^t} ((T-t) \cdot \sum_{k=1}^n p_k r_k F_k(r_k \mu_{t+1}(\mathbf{c}^t))) = (T-t) \cdot \sum_{k=1}^n p_k r_k^2 f_k(r_k \mu_{t+1}(\mathbf{c}^t)) \cdot \frac{\partial \mu_{t+1}(\mathbf{c}^t)}{\partial c_{jt}^t} = \frac{1}{\mu_{t+1}(\mathbf{c}^t)}$$

which implies that

$$(T-t) \cdot \sum_{k=1}^n p_k r_k \cdot (F_k(r_k \mu_{t+1}(\mathbf{c}^t)) - F_k(r_k \mu_{t+1}(\mathbf{c}^t - w_i \cdot \mathbf{e}_{j_t}))) = \int_{c_{jt}^t - w_i}^{c_{jt}^t} \frac{1}{\mu_{t+1}(\mathbf{c}^t(u))} du$$

where  $\mathbf{c}^t(u) = \mathbf{c}^t + (u - c_{jt}^t) \cdot \mathbf{e}_{j_t}$ . Also from Lemma 7,  $1/\mu_{t+1}(\mathbf{c}^t)$  is convex over  $c_{jt}^t$  for any  $\mathbf{c}^t$ , then we have that:

$$(T-t) \cdot \sum_{k=1}^n p_k r_k \cdot (F_k(r_k \mu_{t+1}(\mathbf{c}^t)) - F_k(r_k \mu_{t+1}(\mathbf{c}^t - w_i \cdot \mathbf{e}_{j_t}))) \leq \frac{w_i}{2} \cdot \left[ \frac{1}{\mu_{t+1}(\mathbf{c}^t)} + \frac{1}{\mu_{t+1}(\mathbf{c}^t - w_i \cdot \mathbf{e}_{j_t})} \right]$$

Define a function  $g(w_i)$  as

$$g(w_i) := \frac{T-t}{w_i^2} \cdot \sum_{k=1}^n p_k r_k \cdot (F_k(r_k \mu_{t+1}(\mathbf{c}^t)) - F_k(r_k \mu_{t+1}(\mathbf{c}^t - w_i \cdot \mathbf{e}_{j_t}))) - \frac{1}{w_i \cdot \mu_{t+1}(\mathbf{c}^t)}$$

then we have that

$$\begin{aligned} g'(w_i) &= -\frac{2(T-t)}{w_i^3} \cdot \sum_{k=1}^n p_k r_k \cdot (F_k(r_k \mu_{t+1}(\mathbf{c}^t)) - F_k(r_k \mu_{t+1}(\mathbf{c}^t - w_i \cdot \mathbf{e}_{j_t}))) + \frac{1}{w_i^2 \cdot \mu_{t+1}(\mathbf{c}^t - w_i \cdot \mathbf{e}_{j_t})} + \frac{1}{w_i^2 \cdot \mu_{t+1}(\mathbf{c}^t)} \\ &= -\frac{2}{w_i^3} \cdot \left[ (T-t) \sum_{k=1}^n p_k r_k (F_k(r_k \mu_{t+1}(\mathbf{c}^t)) - F_k(r_k \mu_{t+1}(\mathbf{c}^t - w_i \cdot \mathbf{e}_{j_t}))) - \frac{w_i}{2} \left( \frac{1}{\mu_{t+1}(\mathbf{c}^t)} + \frac{1}{\mu_{t+1}(\mathbf{c}^t - w_i \cdot \mathbf{e}_{j_t})} \right) \right] \\ &\geq 0 \end{aligned}$$

Thus,  $g(w_i)$  is non-decreasing over  $w_i$ , which implies that, for any  $w_i \leq c_{jt}^t$ , we have

$$\begin{aligned} g(w_i) &= \frac{T-t}{w_i^2} \cdot \sum_{k=1}^n p_k r_k \cdot (F_k(r_k \mu_{t+1}(\mathbf{c}^t)) - F_k(r_k \mu_{t+1}(\mathbf{c}^t - w_i \cdot \mathbf{e}_{j_t}))) - \frac{1}{w_i \cdot \mu_{t+1}(\mathbf{c}^t)} \\ &\leq g(c_{jt}^t) = \frac{T-t}{(c_{jt}^t)^2} \cdot \sum_{k=1}^n p_k r_k \cdot (F_k(r_k \mu_{t+1}(\mathbf{c}^t)) - F_k(r_k \mu_{t+1}(\mathbf{c}^t - c_{jt}^t \cdot \mathbf{e}_{j_t}))) - \frac{1}{c_{jt}^t \cdot \mu_{t+1}(\mathbf{c}^t)} \end{aligned}$$

which implies

$$\begin{aligned} & (T-t) \cdot \sum_{k=1}^n p_k r_k \cdot (F_k(r_k \mu_{t+1}(\mathbf{c}^t)) - F_k(r_k \mu_{t+1}(\mathbf{c}^t - w_i \cdot \mathbf{e}_{j_t}))) \\ & \leq \frac{w_i^2 (T-t)}{(c_{j_t}^t)^2} \cdot \sum_{k=1}^n p_k r_k \cdot (F_k(r_k \mu_{t+1}(\mathbf{c}^t)) - F_k(r_k \mu_{t+1}(\mathbf{c}^t - c_{j_t}^t \cdot \mathbf{e}_{j_t}))) + \frac{1}{\mu_{t+1}(\mathbf{c}^t)} \cdot [w_i - \frac{w_i^2}{c_{j_t}^t}] \end{aligned} \quad (87)$$

Also note that from Lemma 3, for each  $i$ , we have that

$$\frac{r_i \mu_{t+1}(\mathbf{c}^t) \cdot (F_i(r_i \mu_{t+1}(\mathbf{c}^t)) - F_i(r_i \mu_{t+1}(\mathbf{c}^t - c_{j_t}^t \cdot \mathbf{e}_{j_t})))}{\int_{r_i \mu_{t+1}(\mathbf{c}^t - c_{j_t}^t \cdot \mathbf{e}_{j_t})}^{r_i \mu_{t+1}(\mathbf{c}^t)} u_i dF_i(u_i)} \leq M$$

which leads to

$$\frac{\sum_{i=1}^n p_i r_i \mu_{t+1}(\mathbf{c}^t) \cdot (F_i(r_i \mu_{t+1}(\mathbf{c}^t)) - F_i(r_i \mu_{t+1}(\mathbf{c}^t - c_{j_t}^t \cdot \mathbf{e}_{j_t})))}{\sum_{i=1}^n p_i \cdot \int_{r_i \mu_{t+1}(\mathbf{c}^t - c_{j_t}^t \cdot \mathbf{e}_{j_t})}^{r_i \mu_{t+1}(\mathbf{c}^t)} u_i dF_i(u_i)} \leq M$$

And from the definition of the threshold  $\mu_t(\mathbf{c}^t)$  in (39), we have

$$\sum_{i=1}^n p_i \cdot \int_{r_i \mu_{t+1}(\mathbf{c}^t - c_{j_t}^t \cdot \mathbf{e}_{j_t})}^{r_i \mu_{t+1}(\mathbf{c}^t)} u_i dF_i(u_i) = \frac{c_{j_t}^t}{T-t}$$

Thus, we have that

$$\sum_{i=1}^n p_i r_i \cdot (F_i(r_i \mu_{t+1}(\mathbf{c}^t)) - F_i(r_i \mu_{t+1}(\mathbf{c}^t - c_{j_t}^t \cdot \mathbf{e}_{j_t}))) \leq \frac{M \cdot c_{j_t}^t}{\mu_{t+1}(\mathbf{c}^t) \cdot (T-t)} \quad (88)$$

Substituting (88) into (87), we have that

$$\begin{aligned} & (T-t) \cdot \sum_{k=1}^n p_k r_k \cdot (F_k(r_k \mu_{t+1}(\mathbf{c}^t)) - F_k(r_k \mu_{t+1}(\mathbf{c}^t - w_i \cdot \mathbf{e}_{j_t}))) \\ & \leq \frac{(M-1) \cdot w_i^2}{\mu_{t+1}(\mathbf{c}^t) \cdot c_{j_t}^t} + \frac{w_i}{\mu_{t+1}(\mathbf{c}^t)} \end{aligned}$$

As a result, we could bound the term III by:

$$\begin{aligned} \text{III} &= \sum_{i=1}^n p_i \cdot \int_0^{h_t^i(\mathbf{c}^t)} \{ (T-t) \cdot \sum_{k=1}^n p_k r_k \cdot (F_k(r_k \mu_{t+1}(\mathbf{c}^t)) - F_k(r_k \mu_{t+1}(\mathbf{c}^t - w_i \cdot \mathbf{e}_{j_t}))) \} dF_i(w_i) \\ & \leq \underbrace{\frac{M-1}{\mu_{t+1}(\mathbf{c}^t) \cdot c_{j_t}^t} \cdot \left[ \sum_{i=1}^n p_i \cdot \int_0^{h_t^i(\mathbf{c}^t)} w_i^2 dF_i(w_i) \right]}_{\text{IV}} + \underbrace{\frac{1}{\mu_{t+1}(\mathbf{c}^t)} \cdot \left[ \sum_{i=1}^n p_i \cdot \int_0^{h_t^i(\mathbf{c}^t)} w_i dF_i(w_i) \right]}_{\text{V}} \end{aligned}$$

In what follows, we upper bound the term IV and V separately and we then get the upper bound of III. Note that

$$\begin{aligned} \sum_{i=1}^n p_i \cdot \int_0^{h_t^i(\mathbf{c}^t)} w_i^2 dF_i(w_i) & \leq \sum_{i=1}^n p_i h_t^i(\mathbf{c}^t) \cdot \int_0^{h_t^i(\mathbf{c}^t)} w_i dF_i(w_i) \leq r_{\max} \cdot \mu_t(\mathbf{c}^t) \cdot \sum_{i=1}^n p_i \cdot \int_0^{h_t^i(\mathbf{c}^t)} w_i dF_i(w_i) \\ & \leq r_{\max} \cdot \mu_t(\mathbf{c}^t) \cdot \sum_{i=1}^n p_i \cdot \int_0^{r_i \mu_t(\mathbf{c}^t)} w_i dF_i(w_i) = r_{\max} \cdot \mu_t(\mathbf{c}^t) \cdot \frac{c_1^t + \dots + c_m^t}{T-t+1} \\ & \leq r_{\max} \cdot \mu_{t+1}(\mathbf{c}^t) \cdot \frac{c_1^t + \dots + c_m^t}{T-t+1} \end{aligned}$$

Thus, we have

$$\text{IV} = \frac{M-1}{\mu_{t+1}(\mathbf{c}^t) \cdot c_{jt}^t} \cdot \left[ \sum_{i=1}^n p_i \cdot \int_0^{h_t^i(\mathbf{c}^t)} w_i^2 dF_i(w_i) \right] \leq \frac{(M-1) \cdot r_{\max} \cdot (c_1^t + \dots + c_m^t)}{c_{jt}^t \cdot (T-t+1)} \leq \frac{(M-1)r_{\max}m}{T-t+1}$$

It also holds that

$$\begin{aligned} \text{V} &= \frac{1}{\mu_{t+1}(\mathbf{c}^t)} \cdot \left[ \sum_{i=1}^n p_i \cdot \int_0^{h_t^i(\mathbf{c}^t)} w_i dF_i(w_i) \right] \leq \frac{1}{\mu_{t+1}(\mathbf{c}^t)} \cdot \left[ \sum_{i=1}^n p_i \cdot \int_0^{r_i \mu_t(\mathbf{c}^t)} w_i dF_i(w_i) \right] \\ &= \frac{c_1^t + \dots + c_m^t}{\mu_{t+1}(\mathbf{c}^t) \cdot (T-t+1)} \end{aligned}$$

Then, we obtain the following upper bound of the term III:

$$\text{III} \leq \frac{(M-1)r_{\max}m}{T-t+1} + \frac{c_1^t + \dots + c_m^t}{\mu_{t+1}(\mathbf{c}^t) \cdot (T-t+1)}$$

Thus, we have

$$\begin{aligned} \rho_t(\mathbf{c}^t) - \bar{\rho}_{t+1} &\leq \text{I} + \text{II} + \text{III} \leq \frac{Mr_{\max}m}{T-t+1} - \frac{c_1^t + \dots + c_m^t}{\mu_{t+1}(\mathbf{c}^t) \cdot (T-t+1)} + \frac{(M-1)r_{\max}m}{T-t+1} + \frac{c_1^t + \dots + c_m^t}{\mu_{t+1}(\mathbf{c}^t) \cdot (T-t+1)} \\ &= \frac{(2mM-m) \cdot r_{\max}}{T-t+1} \end{aligned}$$

holds for all possible  $\mathbf{c}^t$ , which implies that

$$\bar{\rho}_t - \bar{\rho}_{t+1} \leq \frac{(2mM-m) \cdot r_{\max}}{T-t+1}$$

Moreover, noting that  $\bar{\rho}_{T-\hat{K}+1} \leq r_{\max} \cdot \hat{K}$ , we have that

$$\begin{aligned} \rho_1(\mathbf{c}) &\leq \bar{\rho}_1 \leq \sum_{t=1}^{T-\hat{K}} (\bar{\rho}_t - \bar{\rho}_{t+1}) + \bar{\rho}_{T-\hat{K}+1} \leq \sum_{t=1}^{T-\hat{K}} \frac{(2mM-m) \cdot r_{\max}}{T-t+1} + r_{\max} \cdot \hat{K} \\ &\leq (\log T + 1) \cdot (2mM-m) \cdot r_{\max} + r_{\max} \cdot \hat{K} \end{aligned}$$

which completes our proof.
